# Supplementary material for: Dark matter stars
Source: arXiv:2203.12181 ancillary file (2022-03-24)
Supplement: Supplementary file 1 [file Numerical_solution.pdf]

# Numerical solution of the TOV equations for CGF stars

This Sagemath notebook does calculations for the paper *Dark matter stars*.

## Preamble

```
In [1]: %display latex
LE = lambda latex_string: LatexExpr(latex_string);
```

```
In [2]: from timeit import default_timer as timer
# start=timer()
# end=timer()
```

```
In [3]: from mpmath import mp
from mpmath import mpf, mpc
import sage.libs.mpmath.all as a
mp.pretty = True
```

## Code to set floating point precision

**mpf(x)** converts sage floating point numbers to mp numbers

**Reals(x)** or **myR(x)** converts mp numbers to sage

setting **mp.dps** tells mpmath to use decimal precision **mp.dps** or a small amount more

Sagemath decimal precision is set to mpmath decimal precision + 3

```
In [4]: def set_precision(decimal_precision=20):
    global RealNumber, Reals, myR, sage_binary_precision, sage_decimal_precision
    mp.dps = decimal_precision
    binary_precision = mp.prec
    sage_binary_precision = binary_precision + 10
    sage_decimal_precision = floor(sage_binary_precision / log(10, 2))
    Reals = RealField(sage_binary_precision)
    RealNumber = Reals
    myR = Reals
    pretty_print("mp.dps = ", mp.dps, "    mp decimal precision = ", floor(mp.prec / log(10, 2)), "\n"
                "                sage decimal precision = ", sage_decimal_precision )
    set_precision(decimal_precision=20)
```

mp.dps =20      mp decimal precision =21      sage decimal precision =24

## Numerical parameters

Copied from *A theory of the dark matter*

```
In [5]: rhohat_EW_val = 7.974153922874089
c_b_val = 0.24289366755876735
#
g2_val = 0.4262847210445738
lambda_val = 0.5080829235055462
#
lam2_val = lambda_val^2
rhohat_EW_inv_val = 1/rhohat_EW_val
#
rhohat_EW_mpf = mpf(7.974153922874089)
c_a_val = 0.9924810876684255
```

CGF scale

```
In [6]: m, kg, J, GeV, Mpc, pc, km = var('m, kg, J, GeV, Mpc, pc, km')
s = var('s', domain='positive'); assume(s, 'real')
G = RDF(6.67430e-11) * m^3 * kg^(-1) * s^(-2)
c = RDF(2.99792458e8) * m * s^(-1)
hbar = RDF(1.054571817e-34) * J * s
```

```

H0      = RDF(6.74e1) *km * s^(-1) * Mpc^(-1)
Msun    = RDF(1.9884e30)*kg
GMsun   = RDF(1.3271244e20)*m^3/s^2
m_Higgs = RDF(125.10)*GeV
#
J_per_GeV = RDF(1e9*1.602176634e-19)*J/GeV
J_per_kg  = RDF(2.99792458e8^2) *J/kg
m_per_pc  = RDF(3.085677581 * 1e16) * m/pc
GeV_per_kg = J_per_kg/J_per_GeV
pc_per_Mpc = RDF(1e6) *pc/Mpc
m_per_km  = RDF(1e3) *m/km
#
m_Higgs_kg = m_Higgs/GeV_per_kg
#
rho_b = m_Higgs_kg^4/(hbar*c/J_per_kg )^3
r_b_s= (4*RDF(pi)*G*rho_b)^(-1/2)
r_b_m = r_b_s*c
m_b_kg = (r_b_m/G)*c^2
m_b_J = m_b_kg*J_per_kg
m_b_solar = m_b_kg/Msun
pretty_print(LE(r"\frac{G M_S}{G} = "),GMsun/G)
pretty_print(LE(r"\rho_b = "),rho_b)
pretty_print(LE(r"r_b = "),r_b_s,LE(r" = "),r_b_m)
pretty_print(LE(r"m_b = "),m_b_kg,LE(r" = "),m_b_solar,LE(r"M_{\odot} = "), m_b_J)
#print("rho_b = ", rho_b)
#print("r_b = ", r_b_s, " = ", r_b)
#print("m_b = ", m_b, " = ", m_b_J)

```

$$\frac{GM_S}{G} = 1.988409870698051 \times 10^{30} \text{ kg}$$

$$\rho_b = \frac{5.682491786274899 \times 10^{28} \text{ kg}}{m^3}$$

$$r_b = (1.4485143361532907 \times 10^{-10}) \text{ s} = 0.04342536732836333 \text{ m}$$

$$m_b = 5.84762054071815 \times 10^{25} \text{ kg} = 2.9408673007031534 \times 10^{-05} M_{\odot} = 5.255579244258227 \times 10^{42} \text{ J}$$

In [7]:

```

pretty_print(LE(r"c_a= "), RDF(c_a_val),\
              LE(r"\quad \pi c_a^{1/2} = "), RDF(pi*c_a_val^(1/2)),\
              LE(r"\quad \pi c_a^{3/2} = "), RDF(pi*c_a_val^(3/2)))
pretty_print(LE(r"\frac{3\pi c_a^{5/2}}{4} = "), RDF(3*pi*c_a_val^(5/2)/4))

```

$$c_a = 0.9924810876684255 \quad \pi c_a^{1/2} = 3.1297596889937487 \quad \pi c_a^{3/2} = 3.1062273002733085$$

$$\frac{3\pi c_a^{5/2}}{4} = 2.312153887140458$$

## Code

The TOV equations form an ode with independent variable  $\hat{r}$  and dependent variables  $\hat{p}$ ,  $\hat{m}$ ,  $\hat{e}$ .

There are two odes:

- an ode for the core, using the high density equation of state,
- an ode for the outer shell, using the low density equation of state.

## TOV equations

In [8]:

```

m, E_tot, rho,p,r,G= var('m,E_tot,rho,p,r,G')
dpdr_sym = var('dpdr_sym',latex_name=r"\frac{dp}{dr}")
dmdr_sym = var('dmdr_sym',latex_name=r"\frac{dm}{dr}")
dEdr_sym = var('dEdr_sym',latex_name=r"\frac{dE_{tot}}{dr}")
#
dpdr = -(rho+p)*(G*m+4*pi*G*r^3*p)/(r*(r-2*G*m)); dpdr
dmdr = 4*pi*r^2*rho
dEdr = 4*pi*rho*r^2*(r/(r-2*G*m))^(1/2)

```

```
#dEdr = 4*pi*rho*r^2*sqrt(r/(r-2*G*m))
pretty_print(LE(r"\text{TOV equations} \quad"),\
    dpdr_sym," = ",dpdr,LE(r"\quad"), dmdr_sym," = ",dmdr,LE(r"\quad"),dEdr_sym," = ",dEdr)
```

$$\text{TOV equations} \quad \frac{dp}{dr} = \frac{(4\pi G p r^3 + Gm)(p + \rho)}{(2Gm - r)r} \quad \frac{dm}{dr} = 4\pi r^2 \rho \quad \frac{dE_{tot}}{dr} = 4\pi r^2 \rho \sqrt{-\frac{r}{2Gm - r}}$$

In [9]:

```
mhat = var('mhat', latex_name=r"\hat m")
phat = var('phat', latex_name=r"\hat p")
rhoat = var('rhoat', latex_name=r"\hat \rho")
rhat = var('rhat', latex_name=r"\hat r")
ehat = var('ehat', latex_name=r"\hat e")
r_b,m_b= var('r_b,m_b')
dmhatdrhat_sym = var('dmhatdrhat_sym', latex_name=r"\frac{d\hat m}{d\hat r}")
dehatdrhat_sym = var('dehatdrhat_sym', latex_name=r"\frac{d\hat e}{d\hat r}")
dphatdrhat_sym = var('dphatdrhat_sym', latex_name=r"\frac{d\hat p}{d\hat r}")
#
rho = rhoat/(4*pi*G*r_b^2)
p = phat/(4*pi*G*r_b^2)
m = mhat*r_b/G
E_tot = ehat *r_b/G
r = rhat*r_b
pretty_print(LE(r"\text{change to dimensionless variables}\quad"),\
    LE(r"r = "),r,LE(r"\quad \rho = "),rho,LE(r"\quad p = "),p,\
    LE(r"\quad m = "),m,LE(r"\quad E_{tot} = "),E_tot)
print('\n')
#
dmhatdrhat = dmdr.subs(m=m,p=p,rho=rho,r=r) * diff(r,rhat)/diff(m,mhat)
dphatdrhat = (dpdr.subs(m=m,p=p,rho=rho,r=r) * diff(r,rhat)/diff(p,phat)).simplify_full()
dehatdrhat = (dEdr.subs(m=m,p=p,rho=rho,r=r) * diff(r,rhat)/diff(E_tot,ehat)).simplify_full()
pretty_print(LE(r"\text{dimensionless TOV equations}\quad"),\
    dphatdrhat_sym," = ",dphatdrhat, LE(r"\quad"),\
    dmhatdrhat_sym," = ",dmhatdrhat,LE(r"\quad"),\
    dehatdrhat_sym," = ",dehatdrhat)
```

$$\text{change to dimensionless variables} \quad r = r_b \hat{r} \quad \rho = \frac{\hat{\rho}}{4\pi G r_b^2} \quad p = \frac{\hat{p}}{4\pi G r_b^2} \quad m = \frac{\hat{m} r_b}{G} \quad E_{tot} = \frac{\hat{E} r_b}{G}$$

$$\text{dimensionless TOV equations} \quad \frac{d\hat{p}}{d\hat{r}} = \frac{\hat{p}^2 \hat{r}^3 + \hat{m} \hat{p} + (\hat{p} \hat{r}^3 + \hat{m}) \hat{\rho}}{2 \hat{m} \hat{r} - \hat{r}^2} \quad \frac{d\hat{m}}{d\hat{r}} = \hat{r}^2 \hat{\rho} \quad \frac{d\hat{E}}{d\hat{r}} = \hat{r}^2 \hat{\rho} \sqrt{-\frac{\hat{r}}{2 \hat{m} - \hat{r}}}$$

## Prepare the core ode

In [10]:

```
c_b = var('c_b')
rhoat_EW = var('rhoat_EW', latex_name=r"\hat \rho_{EW}")
#
phat = (rhoat - c_b*rhoat_EW)/3
pretty_print(LE(r"\text{high density equation of state}\quad"),LE(r"\hat p = "),phat)
```

$$\text{high density equation of state} \quad \hat{p} = -\frac{1}{3} c_b \hat{\rho}_{EW} + \frac{1}{3} \hat{\rho}$$

In [11]:

```
drhoatdrhat_sym = var('drhoatdrhat_sym', latex_name=r"\frac{d\hat \rho}{d\hat r}")
#
drhoatdrhat = (dphatdrhat.subs(phat=phat)/diff(phat,rhoat)).simplify_rational()
pretty_print(LE(r"\text{substitute for }\hat p\quad"),\
    drhoatdrhat_sym," = ",drhoatdrhat)
```

$$\text{substitute for } \hat{p} \quad \frac{d\hat{\rho}}{d\hat{r}} = \frac{c_b^2 \hat{r}^3 \hat{\rho}_{EW}^2 + 4 \hat{r}^3 \hat{\rho}^2 + 12 \hat{m} \hat{\rho} - (5 c_b \hat{r}^3 \hat{\rho} + 3 c_b \hat{m}) \hat{\rho}_{EW}}{3 (2 \hat{m} \hat{r} - \hat{r}^2)}$$

change variables

The density  $\hat{\rho}$  decreases monotonically with the radius  $\hat{r}$  so we can take  $\hat{\rho}$  as the independent variable in the ode. This allows integrating the ode from the initial condition  $\hat{\rho}(0)$  down to  $\hat{\rho} = \hat{\rho}_{EW}$  which is the density at the outer surface of the core.

The ode solver wants the independent variable to increase, so we use

$$u = \frac{\hat{\rho}_{EW}}{\hat{\rho}} \quad u_0 \leq u \leq 1$$

as independent variable. To simplify the ode, we change dependent variables to

$$w = \frac{\hat{m}}{\hat{\rho}_{EW} \hat{r}^3} \quad x = \hat{r}^2 \quad z = \frac{\hat{e}}{\hat{\rho}_{EW}}$$

In [12]:

```
rhohat_EW_inv = var('rhohat_EW_inv', latex_name=r"\hat{\rho}_{EW}^{-1}")
u = var('u')
w = var('w')
x = var('x')
z = var('z')
#
dudrhat_sym = var('dudrhat_sym', latex_name=r"\frac{du}{d\hat{r}}")
dwdrhat_sym = var('dwdrhat_sym', latex_name=r"\frac{dw}{d\hat{r}}")
dzdrhat_sym = var('dzdrhat_sym', latex_name=r"\frac{dz}{d\hat{r}}")
dwdx_sym = var('dwdx_sym', latex_name=r"\frac{dw}{dx}")
dzdx_sym = var('dzdx_sym', latex_name=r"\frac{dz}{dx}")
dxdu_sym = var('dxdu_sym', latex_name=r"\frac{dx}{du}")
dwdu_sym = var('dwdu_sym', latex_name=r"\frac{dw}{du}")
dzdu_sym = var('dzdu_sym', latex_name=r"\frac{dz}{du}")
#
mhat = w*rhat^3*rhohat_EW
ehat = z*rhohat_EW
rhohat = rhohat_EW/u
#
dwdrhat = (dmhatdrhat.subs(mhat=mhat, rhohat=rhohat) - diff(mhat, rhat))/diff(mhat, w).simplify_full()
dudrhat = (drhohatdrhat.subs(mhat=mhat, rhohat=rhohat)/diff(rhohat, u)).simplify_full()
dzdrhat = (dehatdrhat.subs(mhat=mhat, rhohat=rhohat)/rhohat_EW).simplify_full()
rhohat_EW = 1/rhohat_EW_inv
dudrhat = (dudrhat.subs(rhohat_EW=rhohat_EW)).simplify_rational()
#pretty_print(dwdrhat_sym, " = ", dwdrhat, LE(r"\quad"), dudrhat_sym, " = ", dudrhat)
#
rhat = sqrt(x)
#
dwdx = ((dwdrhat.subs(rhat=rhat)*diff(rhat, x)).simplify_full()).factor()
dzdx = ((dzdrhat.subs(rhat=rhat)*diff(rhat, x)).simplify_full()).factor()
dxdu = ((1/(dudrhat.subs(rhat=rhat)*diff(rhat, x))).simplify_full()).factor()
pretty_print(LE(r"\hat{\rho} = "), rhohat, LE(r"\quad\hat{r} = "), rhat, LE(r"\quad\hat{m} = "), mhat)
print('\n')
pretty_print(dwdx_sym, " = ", dwdx, LE(r"\quad"), dzdx_sym, " = ", dzdx)
print('\n')
pretty_print(dxdu_sym, " = ", dxdu, LE(r"\quad"), dwdu_sym, " = ", dwdx_sym * dxdu_sym, \
LE(r"\quad"), dzdu_sym, " = ", dzdx_sym * dxdu_sym)
```

$$\hat{\rho} = \frac{\hat{\rho}_{EW}}{u} \quad \hat{r} = \sqrt{x} \quad \hat{m} = \hat{r}^3 \hat{\rho}_{EW} w$$

$$\frac{dw}{dx} = -\frac{3uw-1}{2ux} \quad \frac{dz}{dx} = \frac{\sqrt{x}\sqrt{-\frac{1}{2\hat{\rho}_{EW}wx-1}}}{2u}$$

$$\frac{dx}{du} = -\frac{6(2wx - \hat{\rho}_{EW}^{-1})}{(c_b u - 3uw - 1)(c_b u - 4)} \quad \frac{dw}{du} = \frac{dw}{dx} \frac{dx}{du} \quad \frac{dz}{du} = \frac{dz}{dx} \frac{dx}{du}$$

make ode derivatives into functions callable by the ode solver

$$\frac{dw}{du}, \frac{dx}{du}, \frac{dz}{du}$$

In [13]:

```
dwdu = ((dwdx*dxdu).simplify_full()).factor()
dwdu_num = dwdu.subs(rhohat_EW_inv=rhohat_EW_inv_val, c_b=c_b_val)
```

```

dxdu_num = dxdu.subs(rhohat_EW_inv=rhohat_EW_inv_val,c_b=c_b_val)
#
dwdu_fn=fast_callable(dwdu_num,vars=[u,w,x])
dxdu_fn=fast_callable(dxdu_num,vars=[u,w,x])
#
dzdu_fn = lambda u,w,x: (mp.sqrt(x/(1-2*rhohat_EW_mpf*w*x))/(2*u)) *dxdu_fn(u,w,x)

```

## prepare the initial condition

The ode is singular at  $\hat{r} = 0$  so start the ode at  $u = u_0(1 + \epsilon)$ .

In [14]:

```

uu0,xx,bb_1,aa_1 = var('uu0,xx,bb_1,aa_1')
usubs = uu0*(1+xx)
wsubs = (1+aa_1*xx)/(3*uu0)
xsubs = bb_1*xx
rhs_w = ( ( dwdu.subs(u==usubs,w==wsubs,x== xsubs) ).simplify_rational() ).subs(xx==0)
rhs_x = ( ( dxdu.subs(u==usubs,w==wsubs,x== xsubs) ).simplify_rational() ).subs(xx==0)
sol = solve([diff(wsubs,xx) == rhs_w, diff(xsubs,xx) == rhs_x],aa_1,bb_1,solution_dict=True)
a_1 = sol[0][aa_1]
b_1 = sol[0][bb_1]
pretty_print(LE(r"u = u_0(1+\epsilon)",LE(r"\quad w = \frac{1+a_1\epsilon}{3u_0}",\
LE(r"\quad x = b_1 \epsilon \quad z = \frac{1}{3}\hat{\rho}_0\hat{r}^3 = \frac{x^{3/2}}{3u_0} ")))
print('\n')
pretty_print(LE(r"a_1 = ",a_1,LE(r"\quad b_1 = ",b_1)
a_1_fn = fast_callable(a_1.subs(c_b == c_b_val,rhohat_EW_inv == rhohat_EW_inv_val),vars=[uu0])
b_1_fn = fast_callable(b_1.subs(c_b == c_b_val,rhohat_EW_inv == rhohat_EW_inv_val),vars=[uu0])

```

$$u = u_0(1 + \epsilon) \quad w = \frac{1 + a_1\epsilon}{3u_0} \quad x = b_1\epsilon \quad z = \frac{1}{3}\hat{\rho}_0\hat{r}^3 = \frac{x^{3/2}}{3u_0}$$

$$a_1 = -\frac{3}{5} \quad b_1 = \frac{6\hat{\rho}_{EW}^{-1}}{c_b^2 u_0^2 - 6c_b u_0 + 8}$$

## define a function to convert ode-solver output to star data

The ode-solver outputs  $y=[w,x,z]$ .

The star data is  $(\hat{r}, \hat{m}, \hat{e}, \hat{\rho}, \hat{p})$

In [15]:

```

mhat_wx= mhat.subs(rhat=rhat);mhat_wx
mhat_wx_num= mhat_wx.subs(rhohat_EW = rhohat_EW_val)
mhat_wx_fn = fast_callable(mhat_wx_num,vars=[w,x])
#
rhat_x_fn= fast_callable(rhat,vars=[x])
#
rhohat_num = rhohat.subs(rhohat_EW = rhohat_EW_val); rhohat_num
rhohat_u_fn = fast_callable(rhohat_num,vars=[u])
#
phat1 = phat.subs(rhohat=rhohat)
phat_num= phat1.subs(rhohat_EW=rhohat_EW_val,c_b=c_b_val); phat_num
phat_u_fn = fast_callable(phat_num,vars=[u])
#
pretty_print(LE(r"\hat r = "),rhat,LE(r"\quad\hat m = "),mhat_wx,\
LE(r"\quad\hat e = z \hat{\rho}_{EW}"),LE(r"\quad\hat{\rho} = "),\
rhohat, LE(r"\quad\hat p = "),phat)
#
def rhat_mhat_ehat_rhohat_phat(u,y):
    w=y[0]
    x=y[1]
    z=y[2]
    ehat = z*rhohat_EW_mpf
    return (rhat_x_fn(x),mhat_wx_fn(w,x),ehat,rhohat_u_fn(u),phat_u_fn(u))

```

$$\hat{r} = \sqrt{x} \quad \hat{m} = \hat{\rho}_{EW} w x^{\frac{3}{2}} \quad \hat{e} = z \hat{\rho}_{EW} \quad \hat{\rho} = \frac{\hat{\rho}_{EW}}{u} \quad \hat{p} = -\frac{1}{3} c_b \hat{\rho}_{EW} + \frac{1}{3} \hat{\rho}$$

**(rhohat\_norm\_0\_actual, core\_ode) = make\_core\_ode(rhohat\_norm\_0)**

**rhohat\_norm\_0** =  $\hat{\rho}_{norm}(0)$  is the initial condition at  $\hat{r} = 0$ .

$$\hat{\rho}_{norm} = \frac{\hat{\rho}}{\hat{\rho}_{EW}} = \frac{1}{u}$$

$\text{rhat\_norm\_0\_actual} = (1 - \epsilon)\hat{\rho}_{norm}(0)$  is the actual initial value given to the ode-solver.

$\text{core\_ode} : \hat{\rho}_{norm} \mapsto (\hat{r}, \hat{m}, \hat{e}, \hat{\rho}, \hat{p})$  is the solution of the ode for

$$\hat{\rho}_{norm} \leq (1 - \epsilon)\hat{\rho}_{norm}(0)$$

The actual ode-solver is **[w,x,z] = the\_odefun(u)** for

$$(1 + \epsilon)u_0 \leq u$$

In [16]:

```
ode_tol = None
ode_degree = None
epsilon=mpf(1e-20)
F_core = lambda u,y: [dwdu_fn(u,y[0],y[1]),dxdu_fn(u,y[0],y[1]),dzdu_fn(u,y[0],y[1])]
#
def make_core_ode(rhohat_norm_0):
    rhohat_norm_0_actual = mpf(rhohat_norm_0) - epsilon
    u0 = mpf(1/rhohat_norm_0_actual)
    a_1_val = a_1_fn(u0)
    b_1_val = b_1_fn(u0)
    w0 = mpf((1-a_1_val*epsilon)/(3*u0))
    x0 = mpf(b_1_val*epsilon)
    z0 = mp.power(x0,3/2)/(3*u0)
    the_odefun = mp.odefun(F_core,u0,[w0,x0,z0],tol=ode_tol,degree=ode_degree)
    core_ode = lambda rhohat_norm: rhat_mhat_ehat_rhohat_phat(1/rhohat_norm,\
        the_odefun(1/rhohat_norm))
    return (rhohat_norm_0_actual,core_ode)
```

## Prepare the shell ode

The low density equation of state is expressed implicitly

$$\hat{\rho}, \hat{p} = \hat{\rho}(k^2), \hat{p}(k^2) \quad \frac{1}{2} \geq k^2 \geq 0 \quad \hat{\rho}(1/2) = \hat{\rho}_{EW} \quad \hat{\rho}(0) = 0$$

The functions  $\hat{\rho}(k^2), \hat{p}(k^2)$  are expressed by a series of formulas listed in Table 2 of *A theory of the dark matter*. The formulas involve the the ratio  $K/E$  where  $K(k)$  and  $E(k)$  are the complete elliptic integrals.  $k^2$  is the *elliptic parameter*.

The usual notation is  $m = k^2$ .

The TOV equations are solved with

$$\text{independent variable } \sigma = 1 - 2m \quad \text{dependent variables } \hat{r}, \hat{m}, \hat{e}$$

During the preparation of the ode it is convenient to use

$$s = -\ln m \quad \frac{d}{ds} = -m \frac{d}{dm} = \frac{1-\sigma}{2} \frac{d}{d\sigma}$$

## code to define functions of $m$

The following code enters the Table 2 formulas as SageMath symbolic expressions.

In [17]:

```
latex_name={}
latex_name['alpha2_b2'] = r"\alpha^2\langle b^2\rangle"
latex_name['alpha2_mu2'] = r"\alpha^2\mu^2"
latex_name['alpha4_ECGF'] = r"\alpha^4 E_{\mathrm{EW}}"
latex_name['alpha2_ahat2'] = r"\alpha^2 \hat{a}^2"
latex_name['rhohat'] = r"\hat{\rho}"
latex_name['phat'] = r"\hat{p}"
latex_name['lam2'] = r"\lambda^2"
latex_name['g2'] = r"g^2"
latex_name['EoverK'] = r"\frac{E}{K}"
latex_name['m'] = r"m"
for vstr,form in latex_name.items():
    var(vstr,latex_name=latex_name[vstr])
#
formula={}
formula['alpha2_b2'] = m-1+EoverK
```

```

formula['alpha2_mu2']      = 1-2*m
formula['alpha4_ECGF']     = m*(1-m)/2
formula['alpha2_ahat2']    = 3*alpha2_b2/2 + (4*lam2/g2)*alpha2_mu2
formula['rhat']            = ((3/g2)*alpha4_ECGF+(9/(32*lam2))*alpha2_b2^2)/alpha2_ahat2^2
formula['phat']            = ( (1/g2)*(alpha4_ECGF-alpha2_mu2*alpha2_b2)\
                             - (9/(32*lam2))*alpha2_b2^2 )/alpha2_ahat2^2
pretty_print("formulas from Table 2")
print('\n')
for vstr,form in formula.items():
    pretty_print(LE(latex_name[vstr]),' = ', formula[vstr], hold=True)
print('\n')

```

formulas from Table 2

$$\alpha^2 \langle b^2 \rangle = \frac{E}{K} + m - 1$$

$$\alpha^2 \mu^2 = -2m + 1$$

$$\alpha^4 E_{EW} = -\frac{1}{2}(m-1)m$$

$$\alpha^2 \hat{a}^2 = \frac{3}{2} \alpha^2 \langle b^2 \rangle + \frac{4 \alpha^2 \mu^2 \lambda^2}{g^2}$$

$$\hat{\rho} = \frac{3 \left( \frac{3 \alpha^2 \langle b^2 \rangle^2}{\lambda^2} + \frac{32 \alpha^4 E_{EW}}{g^2} \right)}{32 \alpha^2 \hat{a}^2}$$

$$\hat{p} = - \frac{\frac{9 \alpha^2 \langle b^2 \rangle^2}{\lambda^2} + \frac{32 (\alpha^2 \langle b^2 \rangle \alpha^2 \mu^2 - \alpha^4 E_{EW})}{g^2}}{32 \alpha^2 \hat{a}^2}$$

Next, substitutions are made in the formulas to define functions

$$m, E/K \mapsto \hat{\rho}, \hat{p}, \frac{d\hat{p}}{d\sigma}$$

For efficiency, the elliptic integrals  $E$ ,  $K$  will be calculated separately.

In [18]:

```

expr={}
for var_str in list(formula.keys()):
    formula_expanded = eval(preparse(str(formula[var_str])))
    locals()[var_str] = formula_expanded
    expr[var_str] = formula_expanded

mdot = -m
EoverKdot = 1/2 -EoverK +EoverK^2/(2*(1-m))
dot = lambda y: mdot*y.diff(m) + EoverKdot*y.diff(EoverK)
#
expr['dphatds'] = dphatds = dot(phat)

expr_n={}
for var_str,expre in expr.items():
    expr_n[var_str] = expre.subs(lam2==lam2_val,g2==g2_val)

fast={}
for var_str,expre in expr_n.items():
    fast[var_str] = fast_callable(expre,vars=[m,EoverK])
pretty_print(LE(r"\text{fast_callable versions of}"),list(fast.keys()))

```

fast\_callable versions of  $[\alpha_2, \mu_2, \alpha_4, \hat{\alpha}_2, \rho, \phi, d\phi/ds]$

define functions

$$m \mapsto (\hat{\rho}, \hat{p}, d\hat{p}/ds) \quad m \mapsto (\hat{\rho}, \hat{p})$$

```
In [19]: def rhorhat_phat_dphatds(m_arg):
m_val = mpf(m_arg)
KoverE_val = mp.ellipe(m_val)/mp.ellipk(m_val)
rhorhat_val = fast['rhorhat'](m_val, KoverE_val)
phat_val = fast['phat'](m_val, KoverE_val)
dphatds_val = fast['dphatds'](m_val, KoverE_val)
return (rhorhat_val, phat_val, dphatds_val)
```

```
In [20]: def rhorhat_phat(m_arg):
m_val = mpf(m_arg)
KoverE_val = mp.ellipe(m_val)/mp.ellipk(m_val)
rhorhat_val = fast['rhorhat'](m_val, KoverE_val)
phat_val = fast['phat'](m_val, KoverE_val)
return [rhorhat_val, phat_val]
```

define the function that provides the derivatives of the dependent variables to the ode solver.

$$\sigma, y \mapsto \left[ \frac{d\hat{r}}{d\sigma}, \frac{d\hat{m}}{d\sigma}, \frac{d\hat{e}}{d\sigma} \right]$$

```
In [21]: def F_shell(sigma, y_arg):
rhat = y_arg[0]
mhat = y_arg[1]
m = (1-sigma)/2
(rhorhat, phat, dphatds) = rhorhat_phat_dphatds(m)
drhatds = -dphatds*(rhat-2*mhat)/((rhorhat+phat)*(mhat/rhat+rhat^2*phat))
drhatdsigma = drhatds/(1-sigma)
dmhatdsigma = rhat^2*rhorhat*drhatds/(1-sigma)
dehatdrhat = rhorhat*rhat^2/mp.sqrt(1-2*mhat/rhat)
dehatdsigma = dehatdrhat*drhatdsigma
return [drhatdsigma, dmhatdsigma, dehatdsigma]
```

## How stars are represented

A **star** is generated from an initial condition  $\hat{\rho}_{norm}(0)$ .

For  $\hat{\rho}_{norm}(0) > 1$ , first the **core\_ode** is constructed and solved to the endpoint  $u = 1$  to get the core radius, mass, and energy. These are then used as initial conditions for the **shell\_ode** which is solved to the endpoint  $\sigma = 1$  to get the star radius, mass, and energy.

For  $\hat{\rho}_{norm}(0) \leq 1$ , only the **shell\_ode** is constructed and run.

The results are stored in a **star** which is a dictionary with two keys, 'data' and 'ode'.

- **star['data']** is a dictionary with keys
  - 'central density'
  - 'mass'
  - 'radius'
  - 'energy'
  - 'core mass'
  - 'core radius'
  - 'core energy'
  - 'core density'
  - 'core pressure'
  - 'core profile'
  - 'shell profile'
- **star['ode']** is a dictionary with keys
  - 'core ode'
  - 'shell ode'
  - 'initial value'



Numerical values are mpf floating point numbers. '**core profile**' and '**shell profile**' are not used here. Their values would be the intermediate values of the TOV solution for the star. Here we only calculate at the ode endpoints: the data at the boundary of the core and at the boundary of the star.

## How stars are generated and stored

The object is to generate a set of stars more or less evenly spaced on the star curve in the  $M, R$  plane.

The even space is more or less accomplished by an algorithm.

The data is collected in subsets to allow for twiddling the decimal precision and the spacing parameters.

A subset of stars is called a **star\_set**. This is a dictionary of stars. The dictionary key is the star's initial value converted to a string. The value is a **star**.

- **star\_set[skey] = star**

The **star\_sets** are stored in two lists, one for the stars with cores, the other for the coreless stars.

code to make a store with core

**star = make\_star( $\hat{\rho}_{norm}(0)$ )**

In [22]:

```
key = lambda x : "{:.8e}".format(RDF(x))
```

In [23]:

```
ode_tol = None
ode_degree = None
epsilon=mpf(1e-20)
#
F_core = lambda u,y: [dwdu_fn(u,y[0],y[1]),dxdu_fn(u,y[0],y[1]),dzdu_fn(u,y[0],y[1])]
#
def make_star(rhohat_norm_0_arg,return_ode=False):
    rhohat_norm_0 = mpf(rhohat_norm_0_arg)
    star_key = skey(rhohat_norm_0)
    # make core
    rhohat_norm_0_actual = rhohat_norm_0 - epsilon
    u0 = mpf(1/rhohat_norm_0_actual)
    a_1_val = a_1_fn(u0)
    b_1_val = b_1_fn(u0)
    w0 = mpf((1-a_1_val*epsilon)/(3*u0))
    x0 = mpf(b_1_val*epsilon)
    z0 = mp.power(x0,3/2)/(3*u0)
    the_odefun = mp.odefun(F_core,u0,[w0,x0,z0],tol=ode_tol,degree=ode_degree)
    core_ode = lambda rhohat_norm: \
        rhat_mhat_ehat_rhohat_phat(1/rhohat_norm,the_odefun(1/rhohat_norm))
    core_data = core_ode(1)
    # make shell
    y_init = core_data[0:3]
    shell_odefun = mp.odefun(F_shell,0,y_init,tol=ode_tol,degree=ode_degree)
    shell_ode = lambda m: tuple(shell_odefun(mpf(1-2*m)) + rhohat_phat(m))
    shell_data = shell_ode(0)
    # store star
    data={}
    data['central density'] = rhohat_norm_0*rhohat_EW_mpf
    data['radius'] = shell_data[0]
    data['mass'] = shell_data[1]
    data['energy'] = shell_data[2]
    #
    data['core radius'] = core_data[0]
    data['core mass'] = core_data[1]
    data['core energy'] = core_data[2]
    data['core density'] = core_data[3]
    data['core pressure'] = core_data[4]
    # data['core_profile']=None
    # data['shell_profile']=None
    ode={}
    if return_ode:
        ode['core ode'] = core_ode
        ode['shell ode'] = shell_ode
    ode['initial value'] = rhohat_norm_0_actual
    star={}
    star['star key'] =star_key
    star['data'] =data
```

```

star['ode'] =ode
return star

```

## code to adaptively sample parameter space

The last 3 points are used to calculate the radius of curvature  $A/B$  (radius of the circle passing through the points).

At the beginning of a run, 3 stars have to be generated to initialize the adaptive algorithm.

The spacing in the  $\hat{M}$ - $\hat{R}$  plane to the next point is

$$\frac{A}{A + cB} \epsilon'$$

If the radius of curvature is large, the spacing is  $\epsilon'$ . If the radius of curvature is small, the spacing is  $\frac{A}{cB} \epsilon'$ .

Then linear extrapolation gives the parameter step that will give this spacing.

In [24]:

```

def next():
    q10 = p[1]-p[0]
    q21 = p[2]-p[1]
    n10 = norm(q10)
    n21 = norm(q21)
    n20 = norm(q21+q10)
    A = n10*n21*n20
    B = 2*abs(q10[0]*q21[1]-q10[1]*q21[0])
    # A/B is the radius of curvature
    # 1 try R = A/(A+B)
    # 2 try R = A/(A+0.5*B)
    R = A/(A+0.25*B)
    return R*(t[2]-t[1])/n21

```

In [25]:

```

def initialize_adaptive(rhohat_norms):
    global star_set,p,t
    if len(rhohat_norms) != 3:
        print("ERROR: NEED 3 stars")
        return
    this_star_set={}
    p=[]
    t=[]
    print("star_set[{0}]".format(len(star_set)))
    for rhohat_norm_0 in rhohat_norms:
        start = timer()
        star = make_star(rhohat_norm_0 )
        end = timer()
        star_key = star['star key']
        this_star_set[star_key]=star
        star_data = star['data']
        print_star(star_key,star_data,time=end-start)
        rhat = star_data['radius']
        mhat = star_data['mass']
        p.append(vector([Reals(mhat),Reals(rhat)]))
        t.append(Reals(rhohat_norm_0))
    star_set.append(this_star_set)
def make_stars_adaptive(rhohat_norm_max=10,eps=.1):
    global star_set,p,t
    this_star_set ={}
    print("star_set[{0}]".format(len(star_set)))
    rhohat_norm_0 = t[2]
    while rhohat_norm_0 <= rhohat_norm_max:
        rhohat_norm_0 = rhohat_norm_0+eps*next()
        start = timer()
        star = make_star(rhohat_norm_0)
        end = timer()
        star_key = star['star key']
        this_star_set[star_key]=star
        star_data = star['data']
        print_star(star_key,star_data,time=end-start)
        rhat = star_data['radius']
        mhat = star_data['mass']
        p.append(vector([Reals(mhat),Reals(rhat)]))
        p.pop(0)
        t.append(Reals(rhohat_norm_0))
        t.pop(0)
    star_set.append(this_star_set)

```

## code for coreless stars

For  $\hat{\rho}_{norm}(0) \leq 1$  the star has no core. Only the shell ode is run.

Again  $\hat{r} = 0$  is a singular point of the ode. The initial condition is again shifted by  $\epsilon$ .

$$\begin{aligned}\sigma &= \sigma_0 + \epsilon \\ c_1 &= \hat{r} \frac{d\hat{r}}{d\sigma}_{/\sigma_0} \quad \hat{r}^2 = 2c_1\epsilon \\ \frac{d\hat{p}}{d\hat{r}} &= -(\hat{\rho}_0 + \hat{p}_0) \left( \frac{1}{3}\hat{\rho}_0 + \hat{p}_0 \right) \hat{r} \quad \hat{p} = \hat{p}_0 - \hat{\rho}_0 + \hat{p}_0 \left( \frac{1}{3}\hat{\rho}_0 + \hat{p}_0 \right) \frac{1}{2}\hat{r}^2 \\ \hat{m} = \hat{e} &= \frac{1}{3}\hat{\rho}_0\hat{r}^3\end{aligned}$$

In [26]:

```
ode_tol = None
ode_degree = None
epsilon=mpf(1e-20)
#
#
def make_coreless_star(m_0_arg,return_ode=False):
    if m_0_arg > 1/2:
        print('ERROR: star_key must be <= 1/2')
        return
    m_0 = mpf(m_0_arg)
    # m_0 = mpf(Reals(m_0_arg))
    star_key = skey(m_0)
    #
    (rho_hat_norm_0_actual,phat_s) = rho_hat_phat(m_0)
    rhat_s = var('rhat_s',latex_name=r"\hat{r}")
    (rho_hat_s_mpf,phat_s,dphatds_s) = rho_hat_phat_dphatds(m_0)
    rho_hat_s=Reals(rho_hat_s_mpf)
    phat_s=Reals(phat_s)
    dphatds_s=Reals(dphatds_s)
    mhat_s = rho_hat_s*rhat_s^3/3
    drhatds_s = -dphatds_s*(rhat_s-2*mhat_s)/((rho_hat_s+phat_s)*(mhat_s/rhat_s+rhat_s^2*phat_s))
    c1 = mpf((rhat_s*drhatds_s).simplify_rational().subs(rhat_s =0))
    c1 = mp.sqrt(2*c1)
    #
    m_0_actual = m_0*(1-c1*epsilon*epsilon)
    rhat_init = c1*epsilon
    mhat_init = rho_hat_s*mp.power(rhat_init,3)/3
    ehat_init = mhat_init
    y_init = [rhat_init,mhat_init,ehat_init]
    sigma_init = mpf(1 - 2*m_0_actual)
    shell_odefun = mp.odefun(F_shell,sigma_init,y_init,tol=ode_tol,degree=ode_degree)
    shell_ode = lambda m: tuple(shell_odefun(mpf(1-2*m)) + rho_hat_phat(m))
    shell_data = shell_ode(0)
    # store star
    data={}
    data['central density'] = rho_hat_s_mpf
    data['radius'] = shell_data[0]
    data['mass'] = shell_data[1]
    data['energy'] = shell_data[2]
    # data['shell_profile']=None
    ode={}
    if return_ode:
        ode['shell ode'] = shell_ode
    ode['initial value'] = m_0_actual
    star={}
    star['star key'] =star_key
    star['data'] =data
    star['ode'] =ode
    return star
```

In [27]:

```
def initialize_adaptive_coreless(ms):
    global coreless_star_set,p,t
    if len(ms) != 3:
        print("ERROR: NEED 3 stars")
        return
    this_star_set={}
    p=[]
    t=[]
    print("coreless_star_set[{0}]".format(len(coreless_star_set)))
    for m_0 in ms:
```

```

start = timer()
star = make_coreless_star(m_0)
end = timer()
star_key = star['star key']
this_star_set[star_key]=star
star_data = star['data']
print_star(star_key,star_data,time=end-start)
rhat = star_data['radius']
mhat = star_data['mass']
p.append(vector([Reals(mhat),Reals(rhat)]))
t.append(Reals(m_0))
coreless_star_set.append(this_star_set)
def make_coreless_stars_adaptive(m_min=0.4,eps=.1):
    global coreless_star_set,p,t
    this_star_set ={}
    print("coreless_star_set[{0}]" .format(len(coreless_star_set)))
    m_0 = t[2]
    while m_0 >= m_min:
        m_0 = m_0+eps*next()
        start = timer()
        star = make_coreless_star(m_0)
        end = timer()
        star_key = star['star key']
        this_star_set[star_key]=star
        star_data = star['data']
        print_star(star_key,star_data,time=end-start)
        rhat = star_data['radius']
        mhat = star_data['mass']
        p.append(vector([Reals(mhat),Reals(rhat)]))
        p.pop(0)
        t.append(Reals(m_0))
        t.pop(0)
    coreless_star_set.append(this_star_set)

```

code to initialize the adaptive algorithm from the last 3 stars in a star\_set

```

In [28]: def set_pt(a_star_set):
    global p,t
    pf = []
    tf = []
    for star_key in list(a_star_set.keys())[-3:]:
        star_data = a_star_set[star_key]['data']
        mass = star_data['mass']
        radius = star_data['radius']
        param = a_star_set[star_key]['ode']['initial value']
        tf.append(param)
        pf.append(vector([Reals(mass),Reals(radius)]))
    p = pf
    t = tf

```

code for printing and plotting

```

In [29]: def print_star(star_key,star_data,time=0):
    rhat = star_data['radius']
    mhat = star_data['mass']
    ehat = star_data['energy']
    BE = ehat -mhat
    BEratio = BE/mhat
    print(star_key,"r=%.6e" % rhat, "m=%.6e" % mhat, "e=%.6e" % ehat,"BE=%.6e" % BE, "BE/M=%.6e" % BEratio)
#def print_star(star_key,star_data,time=0):
#    rhat = star_data['radius']
#    mhat = star_data['mass']
#    ehat = star_data['energy']
#    BE = ehat -mhat
#    BEratio = BE/mhat
#    print("'" + star_key + "'", " rhat= %.6e" % rhat, " mhat= %.6e" % mhat, " ehat= %.6e" % ehat, " BE= %.6e" % BE, " BEratio= %.6e" % BEratio)
#    pretty_print("'" + star_key + "'", \
#        LE(r"\quad\hat r = "), "%.6e" % rhat, LE(r"\quad\hat m = "), \
#        "%.6e" % mhat, LE(r"\quad\hat e = "), "%.6e" % ehat, \
#        LE(r"\quad BE = "), "%.6e" % BE, LE(r"\quad BE/\hat m = "), \
#        "%.6e" % BEratio,LE(r"\quad"), 'time = ',round(time,1))

```

```

In [30]: def plots(star_dict,xstr,ystr,joined=True):
    if joined:
        the_plot = list_plot( [[star_data[xstr],star_data[ystr]]\
                                for star_key,star_data in star_dict.items()],\

```

```

        marker=None,plotjoined=True,thickness=0.5)
    else:
        the_plot = list_plot( [[star_data[xstr],star_data[ystr]]\
                               for star_key,star_data in star_dict.items()],\
                               marker='.',size=10)
    return the_plot

```

In [31]:

```

def plot_stars(xstr,ystr):
    return list_plot( [[star_data[xstr],star_data[ystr]]\
                       for star_key,star_data in stars.items()],\
                       marker='.',size=10)
def plot_stars_joined(xstr,ystr):
    return list_plot( [[star_data[xstr],star_data[ystr]]\
                       for star_key,star_data in stars.items()],\
                       marker=None,plotjoined=True,thickness=0.5)

```

In [32]:

```

def plot_coreless_stars(xstr,ystr):
    return list_plot( [[star_data[xstr],star_data[ystr]]\
                       for star_key,star_data in coreless_stars.items()],\
                       marker='.',size=10)
def plot_coreless_stars_joined(xstr,ystr):
    return list_plot( [[star_data[xstr],star_data[ystr]]\
                       for star_key,star_data in coreless_stars.items()],\
                       marker=None,plotjoined=True,thickness=0.5)

```

## Plot equation of state

In [33]:

```

rho_low = lambda m: rhohat_phat(m)[0]
w_low = lambda m: rhohat_phat(m)[1]/ rhohat_phat(m)[0]
# p_low =lambda m: rhohat_phat(m)[1]
#
w_low_density_plot = parametric_plot((rho_low,w_low), (m,1e-6,0.5))
rhohat_max =50
w_high_density_plot = plot(lambda xx: (1-c_b_val*rhohat_EW_val/xx)/3,(rhohat_EW_val, rhohat_max))
#
plt = w_low_density_plot+w_high_density_plot
#plt += text(r"$\hat{\rho}_{EW}$", (rhohat_EW_val-1,-.02),fontsize="large")
plt += text(r"$\hat{\rho}_{EW}$", (rhohat_EW_val+2.5,.24),fontsize="large")
plt += line([(rhohat_EW_val,0),(rhohat_EW_val,0.35)],linestyle="--")
plt +=line([(0,1/3),(rhohat_max,1/3)],linestyle=":")
plt.set_aspect_ratio(2*rhohat_max )
plt.set_axes_range(ymax=.35)
plt.axes_labels([r"$\hat{\rho}$",r"$w=\frac{p}{\rho}$"])
show(plt,fontsize=10,axes_labels_size=1.5)
plt.save('plots/rhohat_w.pdf',dpi=600,fontsize=10,axes_labels_size=1.5)

```

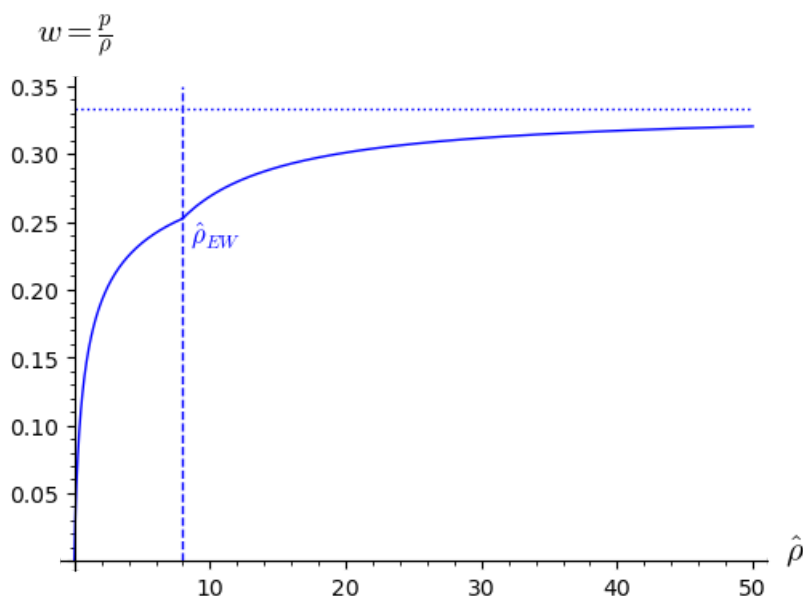

## generate stars with cores

In [34]:

```
star_set=[]
initialize_adaptive([1.0001,1.0011,1.0021])
```

```
star_set[0]
1.00010000e+00 r=1.296425e+00 m=2.324147e-01 e=2.991668e-01 BE=6.675207e-02 BE/M=2.872110e-01 t=9
1.00110000e+00 r=1.296270e+00 m=2.323664e-01 e=2.991125e-01 BE=6.674607e-02 BE/M=2.872449e-01 t=8
1.00210000e+00 r=1.296115e+00 m=2.323182e-01 e=2.990582e-01 BE=6.674008e-02 BE/M=2.872788e-01 t=8
```

In [35]:

```
make_stars_adaptive(rhohat_norm_max=1e9,eps=.02)
```

```
star_set[1]
1.09387377e+00 r=1.282999e+00 m=2.281176e-01 e=2.943168e-01 BE=6.619929e-02 BE/M=2.901981e-01 t=7
1.19720666e+00 r=1.270457e+00 m=2.238962e-01 e=2.895208e-01 BE=6.562456e-02 BE/M=2.931026e-01 t=7
1.31989022e+00 r=1.258032e+00 m=2.194890e-01 e=2.844832e-01 BE=6.499422e-02 BE/M=2.961161e-01 t=6
1.46238263e+00 r=1.246289e+00 m=2.150529e-01 e=2.793804e-01 BE=6.432755e-02 BE/M=2.991243e-01 t=6
1.62513990e+00 r=1.235655e+00 m=2.107082e-01 e=2.743487e-01 BE=6.364054e-02 BE/M=3.020317e-01 t=6
1.80734628e+00 r=1.226476e+00 m=2.065668e-01 e=2.695175e-01 BE=6.295069e-02 BE/M=3.047474e-01 t=6
2.00469227e+00 r=1.219027e+00 m=2.027569e-01 e=2.650390e-01 BE=6.228216e-02 BE/M=3.071765e-01 t=6
2.20742739e+00 r=1.213444e+00 m=1.994188e-01 e=2.610852e-01 BE=6.166636e-02 BE/M=3.092304e-01 t=6
2.40080697e+00 r=1.209636e+00 m=1.966694e-01 e=2.578049e-01 BE=6.113555e-02 BE/M=3.108544e-01 t=6
2.57030402e+00 r=1.207268e+00 m=1.945460e-01 e=2.552554e-01 BE=6.070939e-02 BE/M=3.120567e-01 t=6
2.70870885e+00 r=1.205889e+00 m=1.929808e-01 e=2.533661e-01 BE=6.038533e-02 BE/M=3.129085e-01 t=6
2.81807217e+00 r=1.205100e+00 m=1.918383e-01 e=2.519813e-01 BE=6.014306e-02 BE/M=3.135092e-01 t=6
2.90547009e+00 r=1.204640e+00 m=1.909795e-01 e=2.509370e-01 BE=5.995756e-02 BE/M=3.139477e-01 t=6
2.97813238e+00 r=1.204361e+00 m=1.902994e-01 e=2.501080e-01 BE=5.980852e-02 BE/M=3.142864e-01 t=6
3.04134385e+00 r=1.204191e+00 m=1.897315e-01 e=2.494140e-01 BE=5.968251e-02 BE/M=3.145631e-01 t=6
3.09847348e+00 r=1.204090e+00 m=1.892361e-01 e=2.488075e-01 BE=5.957143e-02 BE/M=3.147996e-01 t=6
3.15162636e+00 r=1.204039e+00 m=1.887898e-01 e=2.482602e-01 BE=5.947039e-02 BE/M=3.150086e-01 t=6
3.20219250e+00 r=1.204027e+00 m=1.883777e-01 e=2.477540e-01 BE=5.937627e-02 BE/M=3.151979e-01 t=6
3.25117434e+00 r=1.204048e+00 m=1.879898e-01 e=2.472767e-01 BE=5.928690e-02 BE/M=3.153730e-01 t=6
3.29936223e+00 r=1.204098e+00 m=1.876185e-01 e=2.468192e-01 BE=5.920066e-02 BE/M=3.155374e-01 t=6
3.34743008e+00 r=1.204176e+00 m=1.872581e-01 e=2.463743e-01 BE=5.911625e-02 BE/M=3.156940e-01 t=6
3.39599293e+00 r=1.204281e+00 m=1.869036e-01 e=2.459362e-01 BE=5.903257e-02 BE/M=3.158450e-01 t=6
3.44564672e+00 r=1.204415e+00 m=1.865508e-01 e=2.454995e-01 BE=5.894862e-02 BE/M=3.159922e-01 t=6
3.49700008e+00 r=1.204581e+00 m=1.861960e-01 e=2.450595e-01 BE=5.886347e-02 BE/M=3.161371e-01 t=6
3.55070333e+00 r=1.204783e+00 m=1.858354e-01 e=2.446115e-01 BE=5.877618e-02 BE/M=3.162809e-01 t=6
3.60747816e+00 r=1.205025e+00 m=1.854653e-01 e=2.441511e-01 BE=5.868580e-02 BE/M=3.164247e-01 t=6
3.66815094e+00 r=1.205316e+00 m=1.850820e-01 e=2.436733e-01 BE=5.859132e-02 BE/M=3.165695e-01 t=6
3.73369229e+00 r=1.205666e+00 m=1.846816e-01 e=2.431733e-01 BE=5.849161e-02 BE/M=3.167159e-01 t=6
3.80526650e+00 r=1.206086e+00 m=1.842599e-01 e=2.426453e-01 BE=5.838543e-02 BE/M=3.168646e-01 t=6
3.88429461e+00 r=1.206594e+00 m=1.838121e-01 e=2.420834e-01 BE=5.827134e-02 BE/M=3.170159e-01 t=6
3.97253631e+00 r=1.207212e+00 m=1.833332e-01 e=2.414809e-01 BE=5.814772e-02 BE/M=3.171697e-01 t=6
4.07219713e+00 r=1.207969e+00 m=1.828176e-01 e=2.408302e-01 BE=5.801267e-02 BE/M=3.173254e-01 t=6
4.18606844e+00 r=1.208905e+00 m=1.822594e-01 e=2.401234e-01 BE=5.786400e-02 BE/M=3.174816e-01 t=6
4.31770840e+00 r=1.210070e+00 m=1.816524e-01 e=2.393516e-01 BE=5.769923e-02 BE/M=3.176354e-01 t=6
4.47166984e+00 r=1.211533e+00 m=1.809907e-01 e=2.385063e-01 BE=5.751560e-02 BE/M=3.177822e-01 t=6
4.65377322e+00 r=1.213386e+00 m=1.802694e-01 e=2.375796e-01 BE=5.731018e-02 BE/M=3.179141e-01 t=6
4.87140319e+00 r=1.215745e+00 m=1.794864e-01 e=2.365665e-01 BE=5.708012e-02 BE/M=3.180193e-01 t=6
5.13376750e+00 r=1.218758e+00 m=1.786440e-01 e=2.354670e-01 BE=5.682309e-02 BE/M=3.180801e-01 t=6
5.45199331e+00 r=1.222605e+00 m=1.777525e-01 e=2.342905e-01 BE=5.653808e-02 BE/M=3.180720e-01 t=6
5.83886659e+00 r=1.227481e+00 m=1.768332e-01 e=2.330596e-01 BE=5.622640e-02 BE/M=3.179629e-01 t=6
6.30801851e+00 r=1.233576e+00 m=1.759208e-01 e=2.318136e-01 BE=5.589272e-02 BE/M=3.177152e-01 t=6
6.87255754e+00 r=1.241032e+00 m=1.750624e-01 e=2.306081e-01 BE=5.554568e-02 BE/M=3.172907e-01 t=6
7.54358866e+00 r=1.249898e+00 m=1.743117e-01 e=2.295090e-01 BE=5.519728e-02 BE/M=3.166585e-01 t=6
8.32946446e+00 r=1.260109e+00 m=1.737197e-01 e=2.285808e-01 BE=5.486106e-02 BE/M=3.158021e-01 t=6
9.23643135e+00 r=1.271494e+00 m=1.733260e-01 e=2.278757e-01 BE=5.454964e-02 BE/M=3.147227e-01 t=6
1.02705121e+01 r=1.283822e+00 m=1.731541e-01 e=2.274269e-01 BE=5.427287e-02 BE/M=3.134369e-01 t=6
1.14397938e+01 r=1.296846e+00 m=1.732126e-01 e=2.272499e-01 BE=5.403726e-02 BE/M=3.119707e-01 t=6
1.27564015e+01 r=1.310337e+00 m=1.735002e-01 e=2.273467e-01 BE=5.384645e-02 BE/M=3.103538e-01 t=6
1.42380027e+01 r=1.324096e+00 m=1.740097e-01 e=2.277118e-01 BE=5.370215e-02 BE/M=3.086159e-01 t=6
1.59091130e+01 r=1.337953e+00 m=1.747317e-01 e=2.283367e-01 BE=5.360505e-02 BE/M=3.067850e-01 t=6
1.78025749e+01 r=1.351762e+00 m=1.756565e-01 e=2.292120e-01 BE=5.355544e-02 BE/M=3.048873e-01 t=6
1.99615229e+01 r=1.365388e+00 m=1.767751e-01 e=2.303287e-01 BE=5.35362e-02 BE/M=3.029477e-01 t=6
2.24420552e+01 r=1.378699e+00 m=1.780787e-01 e=2.316788e-01 BE=5.360013e-02 BE/M=3.009913e-01 t=6
2.53167029e+01 r=1.391559e+00 m=1.795579e-01 e=2.332537e-01 BE=5.369575e-02 BE/M=2.990442e-01 t=6
2.86784664e+01 r=1.403815e+00 m=1.812014e-01 e=2.350428e-01 BE=5.384138e-02 BE/M=2.971356e-01 t=6
3.26442730e+01 r=1.415289e+00 m=1.829929e-01 e=2.370305e-01 BE=5.403761e-02 BE/M=2.952989e-01 t=6
3.73542580e+01 r=1.425770e+00 m=1.849070e-01 e=2.391909e-01 BE=5.428390e-02 BE/M=2.935741e-01 t=6
4.29573337e+01 r=1.435013e+00 m=1.869021e-01 e=2.414790e-01 BE=5.457696e-02 BE/M=2.920083e-01 t=6
4.95617510e+01 r=1.442753e+00 m=1.889113e-01 e=2.438193e-01 BE=5.490798e-02 BE/M=2.906548e-01 t=6
5.71170266e+01 r=1.448756e+00 m=1.908341e-01 e=2.460930e-01 BE=5.525892e-02 BE/M=2.895652e-01 t=6
6.52240279e+01 r=1.452933e+00 m=1.925403e-01 e=2.481405e-01 BE=5.560014e-02 BE/M=2.887714e-01 t=6
7.30377441e+01 r=1.455463e+00 m=1.939078e-01 e=2.498038e-01 BE=5.589598e-02 BE/M=2.882607e-01 t=6
7.95997105e+01 r=1.456794e+00 m=1.948868e-01 e=2.510084e-01 BE=5.612156e-02 BE/M=2.879700e-01 t=6
8.44749070e+01 r=1.457433e+00 m=1.955305e-01 e=2.518073e-01 BE=5.627685e-02 BE/M=2.878163e-01 t=6
8.79138320e+01 r=1.457739e+00 m=1.959469e-01 e=2.523274e-01 BE=5.638056e-02 BE/M=2.877339e-01 t=6
9.04317768e+01 r=1.457898e+00 m=1.962338e-01 e=2.526874e-01 BE=5.645360e-02 BE/M=2.876855e-01 t=6
9.24401777e+01 r=1.457990e+00 m=1.964524e-01 e=2.529626e-01 BE=5.651019e-02 BE/M=2.876533e-01 t=6
9.41737424e+01 r=1.458046e+00 m=1.966343e-01 e=2.531922e-01 BE=5.655787e-02 BE/M=2.876298e-01 t=6
```

|                |                |                |                |                 |                   |     |
|----------------|----------------|----------------|----------------|-----------------|-------------------|-----|
| 9.57508267e+01 | r=1.458079e+00 | m=1.967944e-01 | e=2.533948e-01 | BE=5.660035e-02 | BE/M=2.876116e-01 | t=6 |
| 9.72331598e+01 | r=1.458097e+00 | m=1.969405e-01 | e=2.535800e-01 | BE=5.663952e-02 | BE/M=2.875971e-01 | t=6 |
| 9.86578181e+01 | r=1.458102e+00 | m=1.970770e-01 | e=2.537534e-01 | BE=5.667647e-02 | BE/M=2.875855e-01 | t=6 |
| 1.00051043e+02 | r=1.458096e+00 | m=1.972069e-01 | e=2.539188e-01 | BE=5.671198e-02 | BE/M=2.875761e-01 | t=6 |
| 1.01433959e+02 | r=1.458080e+00 | m=1.973324e-01 | e=2.540790e-01 | BE=5.674663e-02 | BE/M=2.875688e-01 | t=6 |
| 1.02825200e+02 | r=1.458054e+00 | m=1.974554e-01 | e=2.542363e-01 | BE=5.678089e-02 | BE/M=2.875631e-01 | t=6 |
| 1.04242404e+02 | r=1.458019e+00 | m=1.975774e-01 | e=2.543926e-01 | BE=5.681519e-02 | BE/M=2.875592e-01 | t=6 |
| 1.05703277e+02 | r=1.457974e+00 | m=1.976998e-01 | e=2.545497e-01 | BE=5.684993e-02 | BE/M=2.875569e-01 | t=6 |
| 1.07226512e+02 | r=1.457917e+00 | m=1.978239e-01 | e=2.547094e-01 | BE=5.688551e-02 | BE/M=2.875563e-01 | t=6 |
| 1.08832698e+02 | r=1.457847e+00 | m=1.979510e-01 | e=2.548733e-01 | BE=5.692231e-02 | BE/M=2.875576e-01 | t=6 |
| 1.10545321e+02 | r=1.457762e+00 | m=1.980824e-01 | e=2.550432e-01 | BE=5.696079e-02 | BE/M=2.875610e-01 | t=6 |
| 1.12391962e+02 | r=1.457659e+00 | m=1.982196e-01 | e=2.552210e-01 | BE=5.700140e-02 | BE/M=2.875669e-01 | t=6 |
| 1.14405817e+02 | r=1.457535e+00 | m=1.983640e-01 | e=2.554087e-01 | BE=5.704468e-02 | BE/M=2.875758e-01 | t=6 |
| 1.16627676e+02 | r=1.457384e+00 | m=1.985173e-01 | e=2.556086e-01 | BE=5.709127e-02 | BE/M=2.875883e-01 | t=6 |
| 1.19108592e+02 | r=1.457199e+00 | m=1.986815e-01 | e=2.558233e-01 | BE=5.714188e-02 | BE/M=2.876055e-01 | t=6 |
| 1.21913556e+02 | r=1.456973e+00 | m=1.988585e-01 | e=2.560559e-01 | BE=5.719738e-02 | BE/M=2.876285e-01 | t=6 |
| 1.25126617e+02 | r=1.456693e+00 | m=1.990508e-01 | e=2.563096e-01 | BE=5.725881e-02 | BE/M=2.876593e-01 | t=6 |
| 1.28858149e+02 | r=1.456342e+00 | m=1.992610e-01 | e=2.565884e-01 | BE=5.732742e-02 | BE/M=2.877002e-01 | t=6 |
| 1.33255264e+02 | r=1.455901e+00 | m=1.994919e-01 | e=2.568966e-01 | BE=5.740471e-02 | BE/M=2.877546e-01 | t=6 |
| 1.38516899e+02 | r=1.455338e+00 | m=1.997463e-01 | e=2.572388e-01 | BE=5.749244e-02 | BE/M=2.878273e-01 | t=6 |
| 1.44915765e+02 | r=1.454613e+00 | m=2.000268e-01 | e=2.576195e-01 | BE=5.759269e-02 | BE/M=2.879249e-01 | t=6 |
| 1.52830338e+02 | r=1.453671e+00 | m=2.003348e-01 | e=2.580426e-01 | BE=5.770776e-02 | BE/M=2.880566e-01 | t=6 |
| 1.62791105e+02 | r=1.452437e+00 | m=2.006696e-01 | e=2.585097e-01 | BE=5.784003e-02 | BE/M=2.882351e-01 | t=6 |
| 1.75546135e+02 | r=1.450815e+00 | m=2.010264e-01 | e=2.590180e-01 | BE=5.799158e-02 | BE/M=2.884774e-01 | t=6 |
| 1.92150805e+02 | r=1.448685e+00 | m=2.013934e-01 | e=2.595569e-01 | BE=5.816347e-02 | BE/M=2.888053e-01 | t=6 |
| 2.14084225e+02 | r=1.445913e+00 | m=2.017487e-01 | e=2.601033e-01 | BE=5.835465e-02 | BE/M=2.892443e-01 | t=6 |
| 2.43391275e+02 | r=1.442370e+00 | m=2.020581e-01 | e=2.606187e-01 | BE=5.856062e-02 | BE/M=2.898207e-01 | t=6 |
| 2.82851650e+02 | r=1.437973e+00 | m=2.022760e-01 | e=2.610484e-01 | BE=5.877239e-02 | BE/M=2.905554e-01 | t=6 |
| 3.36201516e+02 | r=1.432727e+00 | m=2.023523e-01 | e=2.613290e-01 | BE=5.897673e-02 | BE/M=2.914557e-01 | t=6 |
| 4.08487642e+02 | r=1.426753e+00 | m=2.022428e-01 | e=2.614008e-01 | BE=5.915800e-02 | BE/M=2.925098e-01 | t=6 |
| 5.06689009e+02 | r=1.420281e+00 | m=2.019207e-01 | e=2.612219e-01 | BE=5.930121e-02 | BE/M=2.936857e-01 | t=6 |
| 6.40739085e+02 | r=1.413623e+00 | m=2.013818e-01 | e=2.607765e-01 | BE=5.939468e-02 | BE/M=2.949356e-01 | t=6 |
| 8.24960889e+02 | r=1.407138e+00 | m=2.006463e-01 | e=2.600778e-01 | BE=5.943154e-02 | BE/M=2.962006e-01 | t=6 |
| 1.07945568e+03 | r=1.401208e+00 | m=1.997581e-01 | e=2.591687e-01 | BE=5.941062e-02 | BE/M=2.974128e-01 | t=7 |
| 1.42926102e+03 | r=1.396220e+00 | m=1.987879e-01 | e=2.581255e-01 | BE=5.933762e-02 | BE/M=2.984972e-01 | t=7 |
| 1.89421920e+03 | r=1.392507e+00 | m=1.978352e-01 | e=2.570626e-01 | BE=5.922746e-02 | BE/M=2.993778e-01 | t=7 |
| 2.45685740e+03 | r=1.390212e+00 | m=1.970194e-01 | e=2.561251e-01 | BE=5.910568e-02 | BE/M=2.99992e-01  | t=7 |
| 3.02043700e+03 | r=1.389121e+00 | m=1.964369e-01 | e=2.554393e-01 | BE=5.900239e-02 | BE/M=3.003631e-01 | t=7 |
| 3.44910544e+03 | r=1.388737e+00 | m=1.960988e-01 | e=2.550341e-01 | BE=5.893530e-02 | BE/M=3.005388e-01 | t=7 |
| 3.69953855e+03 | r=1.388627e+00 | m=1.959327e-01 | e=2.548328e-01 | BE=5.890009e-02 | BE/M=3.006139e-01 | t=7 |
| 3.83345744e+03 | r=1.388596e+00 | m=1.958518e-01 | e=2.547341e-01 | BE=5.888235e-02 | BE/M=3.006476e-01 | t=7 |
| 3.91856259e+03 | r=1.388584e+00 | m=1.958030e-01 | e=2.546744e-01 | BE=5.887145e-02 | BE/M=3.006668e-01 | t=7 |
| 3.98729229e+03 | r=1.388578e+00 | m=1.957649e-01 | e=2.546278e-01 | BE=5.886285e-02 | BE/M=3.006813e-01 | t=7 |
| 4.05039293e+03 | r=1.388577e+00 | m=1.957311e-01 | e=2.545862e-01 | BE=5.885511e-02 | BE/M=3.006937e-01 | t=7 |
| 4.11121281e+03 | r=1.388578e+00 | m=1.956994e-01 | e=2.545472e-01 | BE=5.884779e-02 | BE/M=3.007050e-01 | t=7 |
| 4.17114501e+03 | r=1.388581e+00 | m=1.956690e-01 | e=2.545097e-01 | BE=5.884070e-02 | BE/M=3.007155e-01 | t=7 |
| 4.23110830e+03 | r=1.388587e+00 | m=1.956394e-01 | e=2.544731e-01 | BE=5.883374e-02 | BE/M=3.007254e-01 | t=7 |
| 4.29190131e+03 | r=1.388595e+00 | m=1.956102e-01 | e=2.544370e-01 | BE=5.882680e-02 | BE/M=3.007348e-01 | t=7 |
| 4.35430156e+03 | r=1.388606e+00 | m=1.955811e-01 | e=2.544009e-01 | BE=5.881981e-02 | BE/M=3.007439e-01 | t=7 |
| 4.41911471e+03 | r=1.388619e+00 | m=1.955516e-01 | e=2.543643e-01 | BE=5.881268e-02 | BE/M=3.007527e-01 | t=7 |
| 4.48721636e+03 | r=1.388635e+00 | m=1.955216e-01 | e=2.543270e-01 | BE=5.880533e-02 | BE/M=3.007613e-01 | t=7 |
| 4.55959622e+03 | r=1.388655e+00 | m=1.954907e-01 | e=2.542884e-01 | BE=5.879768e-02 | BE/M=3.007697e-01 | t=7 |
| 4.63740995e+03 | r=1.388678e+00 | m=1.954585e-01 | e=2.542481e-01 | BE=5.878962e-02 | BE/M=3.007780e-01 | t=7 |
| 4.72204430e+03 | r=1.388707e+00 | m=1.954247e-01 | e=2.542058e-01 | BE=5.878107e-02 | BE/M=3.007863e-01 | t=7 |
| 4.81520263e+03 | r=1.388742e+00 | m=1.953889e-01 | e=2.541608e-01 | BE=5.877188e-02 | BE/M=3.007944e-01 | t=7 |
| 4.91902107e+03 | r=1.388785e+00 | m=1.953506e-01 | e=2.541125e-01 | BE=5.876192e-02 | BE/M=3.008023e-01 | t=7 |
| 5.03623051e+03 | r=1.388837e+00 | m=1.953094e-01 | e=2.540604e-01 | BE=5.875102e-02 | BE/M=3.008100e-01 | t=7 |
| 5.17038755e+03 | r=1.388902e+00 | m=1.952646e-01 | e=2.540036e-01 | BE=5.873897e-02 | BE/M=3.008173e-01 | t=7 |
| 5.32621095e+03 | r=1.388984e+00 | m=1.952156e-01 | e=2.539411e-01 | BE=5.872551e-02 | BE/M=3.008238e-01 | t=7 |
| 5.51008187e+03 | r=1.389087e+00 | m=1.951617e-01 | e=2.538721e-01 | BE=5.871034e-02 | BE/M=3.008292e-01 | t=7 |
| 5.73080380e+03 | r=1.389219e+00 | m=1.951021e-01 | e=2.537952e-01 | BE=5.869307e-02 | BE/M=3.008326e-01 | t=7 |
| 6.00078208e+03 | r=1.389391e+00 | m=1.950359e-01 | e=2.537092e-01 | BE=5.867325e-02 | BE/M=3.008330e-01 | t=7 |
| 6.33789603e+03 | r=1.389619e+00 | m=1.949627e-01 | e=2.536130e-01 | BE=5.865033e-02 | BE/M=3.008285e-01 | t=7 |
| 6.76853595e+03 | r=1.389923e+00 | m=1.948820e-01 | e=2.535057e-01 | BE=5.862371e-02 | BE/M=3.008164e-01 | t=7 |
| 7.33263347e+03 | r=1.390335e+00 | m=1.947947e-01 | e=2.533874e-01 | BE=5.859274e-02 | BE/M=3.007923e-01 | t=7 |
| 8.09214122e+03 | r=1.390898e+00 | m=1.947034e-01 | e=2.532603e-01 | BE=5.855693e-02 | BE/M=3.007494e-01 | t=7 |
| 9.14549306e+03 | r=1.391672e+00 | m=1.946141e-01 | e=2.531303e-01 | BE=5.851621e-02 | BE/M=3.006781e-01 | t=7 |
| 1.06522953e+04 | r=1.392727e+00 | m=1.945386e-01 | e=2.530101e-01 | BE=5.847151e-02 | BE/M=3.005651e-01 | t=7 |
| 1.28749024e+04 | r=1.394134e+00 | m=1.944960e-01 | e=2.529216e-01 | BE=5.842563e-02 | BE/M=3.003951e-01 | t=7 |
| 1.62460544e+04 | r=1.395933e+00 | m=1.945127e-01 | e=2.528968e-01 | BE=5.838401e-02 | BE/M=3.001552e-01 | t=7 |
| 2.14721895e+04 | r=1.398073e+00 | m=1.946163e-01 | e=2.529710e-01 | BE=5.835464e-02 | BE/M=2.998445e-01 | t=7 |
| 2.96711403e+04 | r=1.400371e+00 | m=1.948211e-01 | e=2.531671e-01 | BE=5.834599e-02 | BE/M=2.994850e-01 | t=7 |
| 4.24746491e+04 | r=1.402521e+00 | m=1.951125e-01 | e=2.534753e-01 | BE=5.836279e-02 | BE/M=2.991237e-01 | t=7 |
| 6.17390691e+04 | r=1.404196e+00 | m=1.954417e-01 | e=2.538435e-01 | BE=5.840178e-02 | BE/M=2.988195e-01 | t=7 |
| 8.78613638e+04 | r=1.405212e+00 | m=1.957388e-01 | e=2.541894e-01 | BE=5.845063e-02 | BE/M=2.986154e-01 | t=7 |
| 1.16332669e+05 | r=1.405649e+00 | m=1.959482e-01 | e=2.544412e-01 | BE=5.849302e-02 | BE/M=2.985127e-01 | t=7 |
| 1.38232288e+05 | r=1.405769e+00 | m=1.960608e-01 | e=2.545799e-01 | BE=5.851914e-02 | BE/M=2.984745e-01 | t=7 |
| 1.49604811e+05 | r=1.405791e+00 | m=1.961078e-01 | e=2.546387e-01 | BE=5.853092e-02 | BE/M=2.984630e-01 | t=7 |
| 1.54479354e+05 | r=1.405794e+00 | m=1.961260e-01 | e=2.546616e-01 | BE=5.853564e-02 | BE/M=2.984594e-01 | t=7 |
| 1.57260978e+05 | r=1.405794e+00 | m=1.961359e-01 | e=2.546742e-01 | BE=5.853826e-02 | BE/M=2.984576e-01 | t=7 |

|                |                |                |                |                 |                   |     |
|----------------|----------------|----------------|----------------|-----------------|-------------------|-----|
| 1.59615424e+05 | r=1.405793e+00 | m=1.961441e-01 | e=2.546845e-01 | BE=5.854042e-02 | BE/M=2.984563e-01 | t=7 |
| 1.61907453e+05 | r=1.405792e+00 | m=1.961518e-01 | e=2.546943e-01 | BE=5.854250e-02 | BE/M=2.984551e-01 | t=7 |
| 1.64212971e+05 | r=1.405790e+00 | m=1.961593e-01 | e=2.547039e-01 | BE=5.854454e-02 | BE/M=2.984540e-01 | t=7 |
| 1.66565743e+05 | r=1.405788e+00 | m=1.961668e-01 | e=2.547134e-01 | BE=5.854659e-02 | BE/M=2.984531e-01 | t=8 |
| 1.68996056e+05 | r=1.405785e+00 | m=1.961744e-01 | e=2.547230e-01 | BE=5.854867e-02 | BE/M=2.984522e-01 | t=7 |
| 1.71535991e+05 | r=1.405781e+00 | m=1.961820e-01 | e=2.547328e-01 | BE=5.855081e-02 | BE/M=2.984514e-01 | t=7 |
| 1.74221205e+05 | r=1.405776e+00 | m=1.961899e-01 | e=2.547429e-01 | BE=5.855302e-02 | BE/M=2.984508e-01 | t=7 |
| 1.77092755e+05 | r=1.405771e+00 | m=1.961980e-01 | e=2.547533e-01 | BE=5.855533e-02 | BE/M=2.984502e-01 | t=7 |
| 1.80199337e+05 | r=1.405764e+00 | m=1.962065e-01 | e=2.547643e-01 | BE=5.855778e-02 | BE/M=2.984497e-01 | t=7 |
| 1.83600187e+05 | r=1.405756e+00 | m=1.962155e-01 | e=2.547759e-01 | BE=5.856039e-02 | BE/M=2.984494e-01 | t=7 |
| 1.87368966e+05 | r=1.405746e+00 | m=1.962250e-01 | e=2.547882e-01 | BE=5.856321e-02 | BE/M=2.984493e-01 | t=7 |
| 1.91599138e+05 | r=1.405734e+00 | m=1.962353e-01 | e=2.548016e-01 | BE=5.856629e-02 | BE/M=2.984493e-01 | t=7 |
| 1.96411582e+05 | r=1.405719e+00 | m=1.962464e-01 | e=2.548161e-01 | BE=5.856968e-02 | BE/M=2.984497e-01 | t=7 |
| 2.01965631e+05 | r=1.405700e+00 | m=1.962585e-01 | e=2.548320e-01 | BE=5.857344e-02 | BE/M=2.984505e-01 | t=7 |
| 2.08475423e+05 | r=1.405677e+00 | m=1.962718e-01 | e=2.548495e-01 | BE=5.857767e-02 | BE/M=2.984518e-01 | t=7 |
| 2.16234679e+05 | r=1.405646e+00 | m=1.962865e-01 | e=2.548690e-01 | BE=5.858247e-02 | BE/M=2.984539e-01 | t=7 |
| 2.25655186e+05 | r=1.405607e+00 | m=1.963029e-01 | e=2.548908e-01 | BE=5.858797e-02 | BE/M=2.984570e-01 | t=7 |
| 2.37328057e+05 | r=1.405556e+00 | m=1.963210e-01 | e=2.549153e-01 | BE=5.859432e-02 | BE/M=2.984618e-01 | t=7 |
| 2.52123935e+05 | r=1.405488e+00 | m=1.963411e-01 | e=2.549428e-01 | BE=5.860170e-02 | BE/M=2.984689e-01 | t=7 |
| 2.71361575e+05 | r=1.405395e+00 | m=1.963631e-01 | e=2.549734e-01 | BE=5.861034e-02 | BE/M=2.984794e-01 | t=8 |
| 2.97099682e+05 | r=1.405269e+00 | m=1.963866e-01 | e=2.550071e-01 | BE=5.862043e-02 | BE/M=2.984950e-01 | t=7 |
| 3.32656335e+05 | r=1.405094e+00 | m=1.964106e-01 | e=2.550427e-01 | BE=5.863213e-02 | BE/M=2.985182e-01 | t=8 |
| 3.83555947e+05 | r=1.404852e+00 | m=1.964326e-01 | e=2.550780e-01 | BE=5.864542e-02 | BE/M=2.985524e-01 | t=8 |
| 4.59282128e+05 | r=1.404520e+00 | m=1.964482e-01 | e=2.551080e-01 | BE=5.865984e-02 | BE/M=2.986021e-01 | t=8 |
| 5.76511989e+05 | r=1.404079e+00 | m=1.964504e-01 | e=2.551246e-01 | BE=5.867420e-02 | BE/M=2.986719e-01 | t=8 |
| 7.64840300e+05 | r=1.403527e+00 | m=1.964301e-01 | e=2.551164e-01 | BE=5.868627e-02 | BE/M=2.987642e-01 | t=8 |
| 1.07562699e+06 | r=1.402902e+00 | m=1.963801e-01 | e=2.550732e-01 | BE=5.869307e-02 | BE/M=2.988748e-01 | t=8 |
| 1.59021594e+06 | r=1.402295e+00 | m=1.963018e-01 | e=2.549940e-01 | BE=5.869218e-02 | BE/M=2.989895e-01 | t=8 |
| 2.40577644e+06 | r=1.401821e+00 | m=1.962100e-01 | e=2.548939e-01 | BE=5.868390e-02 | BE/M=2.990872e-01 | t=8 |
| 3.54163811e+06 | r=1.401548e+00 | m=1.961284e-01 | e=2.548005e-01 | BE=5.867211e-02 | BE/M=2.991516e-01 | t=9 |
| 4.76209689e+06 | r=1.401443e+00 | m=1.960739e-01 | e=2.547358e-01 | BE=5.866197e-02 | BE/M=2.991830e-01 | t=9 |
| 5.64199217e+06 | r=1.401419e+00 | m=1.960468e-01 | e=2.547030e-01 | BE=5.865613e-02 | BE/M=2.991945e-01 | t=9 |
| 6.04996460e+06 | r=1.401417e+00 | m=1.960367e-01 | e=2.546905e-01 | BE=5.865376e-02 | BE/M=2.991978e-01 | t=9 |
| 6.21052475e+06 | r=1.401417e+00 | m=1.960331e-01 | e=2.546859e-01 | BE=5.865288e-02 | BE/M=2.991989e-01 | t=9 |
| 6.30897924e+06 | r=1.401417e+00 | m=1.960309e-01 | e=2.546833e-01 | BE=5.865235e-02 | BE/M=2.991995e-01 | t=9 |
| 6.39966777e+06 | r=1.401417e+00 | m=1.960290e-01 | e=2.546809e-01 | BE=5.865188e-02 | BE/M=2.992000e-01 | t=9 |
| 6.49116536e+06 | r=1.401418e+00 | m=1.960271e-01 | e=2.546785e-01 | BE=5.865141e-02 | BE/M=2.992005e-01 | t=9 |
| 6.58514464e+06 | r=1.401418e+00 | m=1.960252e-01 | e=2.546761e-01 | BE=5.865093e-02 | BE/M=2.992010e-01 | t=9 |
| 6.68281731e+06 | r=1.401419e+00 | m=1.960233e-01 | e=2.546737e-01 | BE=5.865045e-02 | BE/M=2.992014e-01 | t=9 |
| 6.78550817e+06 | r=1.401420e+00 | m=1.960213e-01 | e=2.546713e-01 | BE=5.864995e-02 | BE/M=2.992019e-01 | t=9 |
| 6.89472241e+06 | r=1.401422e+00 | m=1.960193e-01 | e=2.546687e-01 | BE=5.864942e-02 | BE/M=2.992023e-01 | t=8 |
| 7.10222132e+06 | r=1.401423e+00 | m=1.960172e-01 | e=2.546661e-01 | BE=5.864888e-02 | BE/M=2.992027e-01 | t=8 |
| 7.14012303e+06 | r=1.401425e+00 | m=1.960150e-01 | e=2.546633e-01 | BE=5.864829e-02 | BE/M=2.992030e-01 | t=8 |
| 7.28103549e+06 | r=1.401427e+00 | m=1.960127e-01 | e=2.546604e-01 | BE=5.864766e-02 | BE/M=2.992034e-01 | t=8 |
| 7.43823804e+06 | r=1.401430e+00 | m=1.960102e-01 | e=2.546572e-01 | BE=5.864698e-02 | BE/M=2.992037e-01 | t=8 |
| 7.61593594e+06 | r=1.401434e+00 | m=1.960075e-01 | e=2.546537e-01 | BE=5.864624e-02 | BE/M=2.992040e-01 | t=8 |
| 7.81962591e+06 | r=1.401438e+00 | m=1.960046e-01 | e=2.546500e-01 | BE=5.864541e-02 | BE/M=2.992043e-01 | t=8 |
| 8.05663307e+06 | r=1.401443e+00 | m=1.960014e-01 | e=2.546459e-01 | BE=5.864449e-02 | BE/M=2.992045e-01 | t=8 |
| 8.33691772e+06 | r=1.401450e+00 | m=1.959978e-01 | e=2.546413e-01 | BE=5.864345e-02 | BE/M=2.992045e-01 | t=8 |
| 8.67431730e+06 | r=1.401459e+00 | m=1.959939e-01 | e=2.546362e-01 | BE=5.864226e-02 | BE/M=2.992044e-01 | t=8 |
| 9.08850739e+06 | r=1.401470e+00 | m=1.959896e-01 | e=2.546305e-01 | BE=5.864089e-02 | BE/M=2.992041e-01 | t=8 |
| 9.60818449e+06 | r=1.401485e+00 | m=1.959848e-01 | e=2.546241e-01 | BE=5.863930e-02 | BE/M=2.992034e-01 | t=8 |
| 1.02763844e+07 | r=1.401505e+00 | m=1.959794e-01 | e=2.546169e-01 | BE=5.863744e-02 | BE/M=2.992020e-01 | t=8 |
| 1.11596481e+07 | r=1.401533e+00 | m=1.959736e-01 | e=2.546089e-01 | BE=5.863527e-02 | BE/M=2.991998e-01 | t=8 |
| 1.23643236e+07 | r=1.401571e+00 | m=1.959676e-01 | e=2.546003e-01 | BE=5.863274e-02 | BE/M=2.991961e-01 | t=8 |
| 1.40664539e+07 | r=1.401624e+00 | m=1.959617e-01 | e=2.545915e-01 | BE=5.862984e-02 | BE/M=2.991903e-01 | t=8 |
| 1.65679832e+07 | r=1.401698e+00 | m=1.959568e-01 | e=2.545834e-01 | BE=5.862662e-02 | BE/M=2.991813e-01 | t=8 |
| 2.04038101e+07 | r=1.401798e+00 | m=1.959545e-01 | e=2.545778e-01 | BE=5.862329e-02 | BE/M=2.991678e-01 | t=8 |
| 2.65423532e+07 | r=1.401929e+00 | m=1.959571e-01 | e=2.545774e-01 | BE=5.862031e-02 | BE/M=2.991488e-01 | t=8 |
| 3.67301766e+07 | r=1.402085e+00 | m=1.959668e-01 | e=2.545852e-01 | BE=5.861840e-02 | BE/M=2.991242e-01 | t=8 |
| 5.39286695e+07 | r=1.402248e+00 | m=1.959846e-01 | e=2.546030e-01 | BE=5.861833e-02 | BE/M=2.990966e-01 | t=9 |
| 8.22311000e+07 | r=1.402386e+00 | m=1.960079e-01 | e=2.546282e-01 | BE=5.862031e-02 | BE/M=2.990711e-01 | t=9 |
| 1.24208335e+08 | r=1.402474e+00 | m=1.960306e-01 | e=2.546542e-01 | BE=5.862357e-02 | BE/M=2.990532e-01 | t=9 |
| 1.73872855e+08 | r=1.402511e+00 | m=1.960470e-01 | e=2.546736e-01 | BE=5.862666e-02 | BE/M=2.990439e-01 | t=9 |
| 2.14355339e+08 | r=1.402521e+00 | m=1.960557e-01 | e=2.546843e-01 | BE=5.862861e-02 | BE/M=2.990406e-01 | t=9 |
| 2.35086916e+08 | r=1.402522e+00 | m=1.960591e-01 | e=2.546886e-01 | BE=5.862946e-02 | BE/M=2.990397e-01 | t=9 |
| 2.42908309e+08 | r=1.402522e+00 | m=1.960603e-01 | e=2.546901e-01 | BE=5.862975e-02 | BE/M=2.990394e-01 | t=9 |
| 2.46970250e+08 | r=1.402522e+00 | m=1.960609e-01 | e=2.546908e-01 | BE=5.862990e-02 | BE/M=2.990393e-01 | t=9 |
| 2.50525736e+08 | r=1.402522e+00 | m=1.960614e-01 | e=2.546914e-01 | BE=5.863003e-02 | BE/M=2.990392e-01 | t=9 |
| 2.54109072e+08 | r=1.402522e+00 | m=1.960618e-01 | e=2.546920e-01 | BE=5.863016e-02 | BE/M=2.990391e-01 | t=9 |
| 2.57797539e+08 | r=1.402522e+00 | m=1.960623e-01 | e=2.546926e-01 | BE=5.863029e-02 | BE/M=2.990390e-01 | t=9 |
| 2.61638244e+08 | r=1.402521e+00 | m=1.960628e-01 | e=2.546932e-01 | BE=5.863042e-02 | BE/M=2.990390e-01 | t=9 |
| 2.65683716e+08 | r=1.402521e+00 | m=1.960633e-01 | e=2.546939e-01 | BE=5.863055e-02 | BE/M=2.990389e-01 | t=9 |
| 2.69994113e+08 | r=1.402521e+00 | m=1.960638e-01 | e=2.546945e-01 | BE=5.863069e-02 | BE/M=2.990388e-01 | t=9 |
| 2.74640151e+08 | r=1.402520e+00 | m=1.960644e-01 | e=2.546952e-01 | BE=5.863084e-02 | BE/M=2.990388e-01 | t=9 |
| 2.79707214e+08 | r=1.402520e+00 | m=1.960649e-01 | e=2.546959e-01 | BE=5.863100e-02 | BE/M=2.990387e-01 | t=9 |
| 2.85300806e+08 | r=1.402519e+00 | m=1.960655e-01 | e=2.546967e-01 | BE=5.863117e-02 | BE/M=2.990387e-01 | t=9 |
| 2.91554029e+08 | r=1.402519e+00 | m=1.960661e-01 | e=2.546975e-01 | BE=5.863136e-02 | BE/M=2.990386e-01 | t=9 |
| 2.98638112e+08 | r=1.402518e+00 | m=1.960668e-01 | e=2.546984e-01 | BE=5.863156e-02 | BE/M=2.990386e-01 | t=9 |
| 3.06777585e+08 | r=1.402517e+00 | m=1.960676e-01 | e=2.546994e-01 | BE=5.863178e-02 | BE/M=2.990386e-01 | t=9 |



```
3.16272659e+08 r=1.402515e+00 m=1.960684e-01 e=2.547004e-01 BE=5.863204e-02 BE/M=2.990387e-01 t=9
3.27533004e+08 r=1.402513e+00 m=1.960693e-01 e=2.547016e-01 BE=5.863232e-02 BE/M=2.990387e-01 t=9
3.41129972e+08 r=1.402511e+00 m=1.960703e-01 e=2.547030e-01 BE=5.863265e-02 BE/M=2.990389e-01 t=9
3.57879481e+08 r=1.402508e+00 m=1.960715e-01 e=2.547045e-01 BE=5.863302e-02 BE/M=2.990391e-01 t=9
3.78977297e+08 r=1.402504e+00 m=1.960727e-01 e=2.547062e-01 BE=5.863346e-02 BE/M=2.990394e-01 t=9
4.06226515e+08 r=1.402499e+00 m=1.960741e-01 e=2.547080e-01 BE=5.863397e-02 BE/M=2.990399e-01 t=9
4.42432347e+08 r=1.402491e+00 m=1.960755e-01 e=2.547101e-01 BE=5.863457e-02 BE/M=2.990407e-01 t=9
4.92109729e+08 r=1.402481e+00 m=1.960771e-01 e=2.547124e-01 BE=5.863527e-02 BE/M=2.990419e-01 t=9
5.62791377e+08 r=1.402467e+00 m=1.960786e-01 e=2.547146e-01 BE=5.863606e-02 BE/M=2.990437e-01 t=9
6.67508046e+08 r=1.402447e+00 m=1.960797e-01 e=2.547167e-01 BE=5.863695e-02 BE/M=2.990465e-01 t=9
8.29543818e+08 r=1.402421e+00 m=1.960801e-01 e=2.547180e-01 BE=5.863785e-02 BE/M=2.990504e-01 t=9
1.09135005e+09 r=1.402386e+00 m=1.960792e-01 e=2.547179e-01 BE=5.863865e-02 BE/M=2.990559e-01 t=9
```

## generate coreless stars

In [36]:

```
coreless_star_set=[]
initialize_adaptive_coreless([0.5,0.499,0.498])
```

```
coreless_star_set[0]
5.00000000e-01 r=1.296441e+00 m=2.324196e-01 e=2.991722e-01 BE=6.675267e-02 BE/M=2.872076e-01 t=11
4.99000000e-01 r=1.299815e+00 m=2.334598e-01 e=3.003398e-01 BE=6.688004e-02 BE/M=2.864735e-01 t=11
4.98000000e-01 r=1.303226e+00 m=2.344930e-01 e=3.014964e-01 BE=6.700343e-02 BE/M=2.857375e-01 t=11
```

In [37]:

```
make_coreless_stars_adaptive(m_min=0.01,eps=0.025)
```

```
coreless_star_set[1]
4.92774117e-01 r=1.321575e+00 m=2.397770e-01 e=3.073618e-01 BE=6.758479e-02 BE/M=2.818652e-01 t=11
4.87524670e-01 r=1.340742e+00 m=2.448846e-01 e=3.129496e-01 BE=6.806499e-02 BE/M=2.779472e-01 t=11
4.82258661e-01 r=1.360541e+00 m=2.498029e-01 e=3.182499e-01 BE=6.844708e-02 BE/M=2.740044e-01 t=11
4.76928416e-01 r=1.381030e+00 m=2.545698e-01 e=3.233070e-01 BE=6.873718e-02 BE/M=2.700131e-01 t=11
4.7158240e-01 r=1.402020e+00 m=2.591576e-01 e=3.280937e-01 BE=6.893606e-02 BE/M=2.660005e-01 t=11
4.66160607e-01 r=1.423382e+00 m=2.635528e-01 e=3.325991e-01 BE=6.904635e-02 BE/M=2.619830e-01 t=11
4.60741224e-01 r=1.445027e+00 m=2.677497e-01 e=3.368212e-01 BE=6.907144e-02 BE/M=2.579701e-01 t=11
4.55302500e-01 r=1.466891e+00 m=2.717467e-01 e=3.407616e-01 BE=6.901486e-02 BE/M=2.539676e-01 t=11
4.49845040e-01 r=1.488927e+00 m=2.755440e-01 e=3.444241e-01 BE=6.888014e-02 BE/M=2.499788e-01 t=11
4.44368505e-01 r=1.511102e+00 m=2.791426e-01 e=3.478132e-01 BE=6.867064e-02 BE/M=2.460056e-01 t=11
4.38872115e-01 r=1.533388e+00 m=2.825440e-01 e=3.509335e-01 BE=6.838955e-02 BE/M=2.420492e-01 t=11
4.33354925e-01 r=1.555767e+00 m=2.857498e-01 e=3.537897e-01 BE=6.803987e-02 BE/M=2.381100e-01 t=11
4.27815979e-01 r=1.578221e+00 m=2.887613e-01 e=3.563858e-01 BE=6.762447e-02 BE/M=2.341881e-01 t=12
4.22254394e-01 r=1.600738e+00 m=2.915797e-01 e=3.587258e-01 BE=6.714605e-02 BE/M=2.302837e-01 t=12
4.16669397e-01 r=1.623307e+00 m=2.942060e-01 e=3.608132e-01 BE=6.660720e-02 BE/M=2.263964e-01 t=12
4.11060344e-01 r=1.645921e+00 m=2.966410e-01 e=3.626513e-01 BE=6.601039e-02 BE/M=2.225262e-01 t=12
4.05426724e-01 r=1.668571e+00 m=2.988850e-01 e=3.642430e-01 BE=6.535803e-02 BE/M=2.186728e-01 t=12
3.99768157e-01 r=1.691252e+00 m=3.009385e-01 e=3.655909e-01 BE=6.465242e-02 BE/M=2.148360e-01 t=12
3.94084385e-01 r=1.713959e+00 m=3.028016e-01 e=3.666974e-01 BE=6.389584e-02 BE/M=2.110156e-01 t=12
3.88375263e-01 r=1.736686e+00 m=3.044742e-01 e=3.675647e-01 BE=6.309049e-02 BE/M=2.072113e-01 t=12
3.82640754e-01 r=1.759429e+00 m=3.059562e-01 e=3.681948e-01 BE=6.223855e-02 BE/M=2.034230e-01 t=12
3.76880914e-01 r=1.782185e+00 m=3.072474e-01 e=3.685895e-01 BE=6.134214e-02 BE/M=1.996506e-01 t=12
3.71095889e-01 r=1.804951e+00 m=3.083473e-01 e=3.687507e-01 BE=6.040338e-02 BE/M=1.958940e-01 t=13
3.65285904e-01 r=1.827723e+00 m=3.092555e-01 e=3.686798e-01 BE=5.942435e-02 BE/M=1.921529e-01 t=13
3.59451256e-01 r=1.850499e+00 m=3.099714e-01 e=3.683785e-01 BE=5.840713e-02 BE/M=1.884275e-01 t=13
3.53592307e-01 r=1.873276e+00 m=3.104944e-01 e=3.678482e-01 BE=5.735375e-02 BE/M=1.847175e-01 t=13
3.47709480e-01 r=1.896051e+00 m=3.108239e-01 e=3.670901e-01 BE=5.626628e-02 BE/M=1.810230e-01 t=13
3.41803251e-01 r=1.918823e+00 m=3.109591e-01 e=3.661058e-01 BE=5.514674e-02 BE/M=1.773441e-01 t=13
3.35874144e-01 r=1.941588e+00 m=3.108993e-01 e=3.648964e-01 BE=5.399716e-02 BE/M=1.736805e-01 t=13
3.29922729e-01 r=1.964346e+00 m=3.106438e-01 e=3.634633e-01 BE=5.281956e-02 BE/M=1.700326e-01 t=13
3.23949617e-01 r=1.987094e+00 m=3.101917e-01 e=3.618077e-01 BE=5.161595e-02 BE/M=1.664001e-01 t=13
3.17955453e-01 r=2.009829e+00 m=3.095424e-01 e=3.599308e-01 BE=5.038834e-02 BE/M=1.627833e-01 t=13
3.11940916e-01 r=2.032551e+00 m=3.086951e-01 e=3.578338e-01 BE=4.913875e-02 BE/M=1.591822e-01 t=13
3.05906718e-01 r=2.055258e+00 m=3.076489e-01 e=3.555181e-01 BE=4.786918e-02 BE/M=1.555968e-01 t=13
2.99853594e-01 r=2.077947e+00 m=3.064031e-01 e=3.529847e-01 BE=4.658163e-02 BE/M=1.520273e-01 t=13
2.93782307e-01 r=2.100616e+00 m=3.049569e-01 e=3.502350e-01 BE=4.527809e-02 BE/M=1.484737e-01 t=13
2.87693639e-01 r=2.123265e+00 m=3.033097e-01 e=3.472703e-01 BE=4.396057e-02 BE/M=1.449362e-01 t=13
2.81588393e-01 r=2.145892e+00 m=3.014608e-01 e=3.440918e-01 BE=4.263104e-02 BE/M=1.414149e-01 t=12
2.75467392e-01 r=2.168494e+00 m=2.994093e-01 e=3.407008e-01 BE=4.129150e-02 BE/M=1.379099e-01 t=12
2.69331471e-01 r=2.191070e+00 m=2.971548e-01 e=3.370987e-01 BE=3.994392e-02 BE/M=1.344213e-01 t=12
2.63181481e-01 r=2.213619e+00 m=2.946965e-01 e=3.332868e-01 BE=3.859028e-02 BE/M=1.309492e-01 t=12
2.57018284e-01 r=2.236139e+00 m=2.920340e-01 e=3.292665e-01 BE=3.723254e-02 BE/M=1.274939e-01 t=12
2.50842754e-01 r=2.258629e+00 m=2.891666e-01 e=3.250393e-01 BE=3.587265e-02 BE/M=1.240553e-01 t=12
2.44655772e-01 r=2.281086e+00 m=2.860940e-01 e=3.206065e-01 BE=3.451257e-02 BE/M=1.206337e-01 t=12
2.38458228e-01 r=2.303510e+00 m=2.828156e-01 e=3.159698e-01 BE=3.315424e-02 BE/M=1.172292e-01 t=13
2.32251016e-01 r=2.325898e+00 m=2.793310e-01 e=3.111305e-01 BE=3.179957e-02 BE/M=1.138419e-01 t=13
2.26035035e-01 r=2.348250e+00 m=2.756399e-01 e=3.060904e-01 BE=3.045049e-02 BE/M=1.104720e-01 t=13
2.19811190e-01 r=2.370564e+00 m=2.717420e-01 e=3.008509e-01 BE=2.910889e-02 BE/M=1.071196e-01 t=13
2.13580385e-01 r=2.392838e+00 m=2.676370e-01 e=2.954137e-01 BE=2.777667e-02 BE/M=1.037848e-01 t=13
2.07343525e-01 r=2.415071e+00 m=2.633248e-01 e=2.897805e-01 BE=2.645568e-02 BE/M=1.004679e-01 t=13
2.01101517e-01 r=2.437261e+00 m=2.588052e-01 e=2.839530e-01 BE=2.514779e-02 BE/M=9.716879e-02 t=12
1.94855264e-01 r=2.459408e+00 m=2.540782e-01 e=2.779330e-01 BE=2.385483e-02 BE/M=9.388777e-02 t=12
```

```

1.88605668e-01 r=2.481509e+00 m=2.491436e-01 e=2.717222e-01 BE=2.257862e-02 BE/M=9.062493e-02 t=12
1.82353629e-01 r=2.503564e+00 m=2.440016e-01 e=2.653225e-01 BE=2.132095e-02 BE/M=8.738038e-02 t=12
1.76100040e-01 r=2.525570e+00 m=2.386521e-01 e=2.587357e-01 BE=2.008360e-02 BE/M=8.415426e-02 t=12
1.69845791e-01 r=2.547527e+00 m=2.330955e-01 e=2.519638e-01 BE=1.886831e-02 BE/M=8.094669e-02 t=12
1.63591763e-01 r=2.569433e+00 m=2.273318e-01 e=2.450086e-01 BE=1.767682e-02 BE/M=7.775777e-02 t=12
1.57338835e-01 r=2.591286e+00 m=2.213614e-01 e=2.378722e-01 BE=1.651082e-02 BE/M=7.458762e-02 t=12
1.51087873e-01 r=2.613087e+00 m=2.151845e-01 e=2.305565e-01 BE=1.537200e-02 BE/M=7.143635e-02 t=12
1.44839738e-01 r=2.634832e+00 m=2.088016e-01 e=2.230636e-01 BE=1.426200e-02 BE/M=6.830406e-02 t=12
1.38595280e-01 r=2.656522e+00 m=2.022132e-01 e=2.153956e-01 BE=1.318245e-02 BE/M=6.519085e-02 t=12
1.32355341e-01 r=2.678154e+00 m=1.954196e-01 e=2.075545e-01 BE=1.213493e-02 BE/M=6.209682e-02 t=12
1.26120751e-01 r=2.699727e+00 m=1.884215e-01 e=1.995425e-01 BE=1.112102e-02 BE/M=5.902205e-02 t=12
1.19892328e-01 r=2.721241e+00 m=1.812195e-01 e=1.913617e-01 BE=1.014224e-02 BE/M=5.596662e-02 t=12
1.13670881e-01 r=2.742694e+00 m=1.738143e-01 e=1.830144e-01 BE=9.200098e-03 BE/M=5.293062e-02 t=12
1.07457203e-01 r=2.764085e+00 m=1.662066e-01 e=1.745027e-01 BE=8.296056e-03 BE/M=4.991411e-02 t=12
1.01252078e-01 r=2.785412e+00 m=1.583973e-01 e=1.658288e-01 BE=7.431552e-03 BE/M=4.691717e-02 t=12
9.50562739e-02 r=2.806676e+00 m=1.503871e-01 e=1.569951e-01 BE=6.607988e-03 BE/M=4.393985e-02 t=12
8.88705458e-02 r=2.827873e+00 m=1.421771e-01 e=1.480038e-01 BE=5.826732e-03 BE/M=4.098222e-02 t=12
8.26956342e-02 r=2.849004e+00 m=1.337681e-01 e=1.388572e-01 BE=5.089116e-03 BE/M=3.804433e-02 t=12
7.65322651e-02 r=2.870068e+00 m=1.251611e-01 e=1.295576e-01 BE=4.396436e-03 BE/M=3.512621e-02 t=12
7.03811494e-02 r=2.891063e+00 m=1.163574e-01 e=1.201073e-01 BE=3.749955e-03 BE/M=3.222791e-02 t=12
6.42429824e-02 r=2.911988e+00 m=1.073578e-01 e=1.105087e-01 BE=3.150896e-03 BE/M=2.934947e-02 t=12
5.81184438e-02 r=2.932843e+00 m=9.816377e-02 e=1.007642e-01 BE=2.600448e-03 BE/M=2.649091e-02 t=12
5.20081971e-02 r=2.953626e+00 m=8.877635e-02 e=9.087612e-02 BE=2.099761e-03 BE/M=2.365226e-02 t=12
4.59128895e-02 r=2.974337e+00 m=7.919687e-02 e=8.084682e-02 BE=1.649950e-03 BE/M=2.083352e-02 t=12
3.98331516e-02 r=2.994975e+00 m=6.942663e-02 e=7.067872e-02 BE=1.252090e-03 BE/M=1.803472e-02 t=12
3.37695971e-02 r=3.015539e+00 m=5.946698e-02 e=6.037420e-02 BE=9.072200e-04 BE/M=1.525586e-02 t=12
2.77228228e-02 r=3.036027e+00 m=4.931933e-02 e=4.993567e-02 BE=6.163407e-04 BE/M=1.249694e-02 t=12
2.16934077e-02 r=3.056440e+00 m=3.898512e-02 e=3.936553e-02 BE=3.804149e-04 BE/M=9.757953e-03 t=12
1.56819130e-02 r=3.076776e+00 m=2.846582e-02 e=2.866619e-02 BE=2.003678e-04 BE/M=7.038890e-03 t=12
9.68887987e-03 r=3.097035e+00 m=1.776298e-02 e=1.784007e-02 BE=7.708666e-05 BE/M=4.339737e-03 t=12

```

In [38]:

```

set_precision(30)
Rhat_a = Reals(pi*sqrt(c_a_val))
c_M = Reals(pi*c_a_val^(3/2))
c_E = Reals((3*pi/4)*c_a_val^(5/2))
pretty_print(LE(r"\hat R_{asympt} = "), "{:.8f}".format(Rhat_a), \
              LE(r"\qquad\hat M_{asympt} = "), "{:.8f}".format(c_M), LE(r"\:\hat{\rho}(0)"), \
              LE(r"\qquad\hat{B}E_{asympt} = "), "{:.8f}".format(c_E), LE(r"\:\hat{\rho}(0)^2"))
this_star_set = {}
print("coreless_star_set[{0}]".format(len(coreless_star_set)))
for n in range(15):
    m_0 = 5e-3/2^n
    start = timer()
    star = make_coreless_star(m_0)
    end = timer()
    star_key = star['star key']
    this_star_set[star_key] = star
    star_data = star['data']
    print_star(star_key, star_data, time=end-start)
    central_density = Reals(star_data['central density'])
    mass = Reals(star_data['mass'])
    radius = Reals(star_data['radius'])
    energy = Reals(star_data['energy'])
    BE = energy-mass
    pretty_print(LE(r"\frac{R}{R_{asympt}}="), RDF(radius/Rhat_a), \
                LE(r"\qquad\frac{M}{M_{asympt}}="), RDF(mass/(c_M*central_density)), \
                LE(r"\qquad\frac{BE}{BE_{asympt}}="), RDF(BE/(c_E*central_density^2)))
    coreless_star_set.append(this_star_set)
set_precision()

```

mp.dps =30    mp decimal precision =31    sage decimal precision =34

$$\hat{R}_{asympt} = 3.12975969 \quad \hat{M}_{asympt} = 3.10622730 \hat{\rho}(0) \quad \hat{BE}_{asympt} = 2.31215389 \hat{\rho}(0)^2$$

coreless\_star\_set[2]

5.00000000e-03 r=3.112877e+00 m=9.237803e-03 e=9.258458e-03 BE=2.065435e-05 BE/M=2.235851e-03 t=69

$$\frac{R}{R_{asympt}} = 0.9946056049803801 \quad \frac{M}{M_{asympt}} = 0.9796428920439193 \quad \frac{BE}{BE_{asympt}} = 0.9693029209427709$$

2.50000000e-03 r=3.121319e+00 m=4.637931e-03 e=4.643111e-03 BE=5.180341e-06 BE/M=1.116951e-03 t=70

$$\frac{R}{R_{asympt}} = 0.9973031546211996 \quad \frac{M}{M_{asympt}} = 0.9897892048650972 \quad \frac{BE}{BE_{asympt}} = 0.9845660984846787$$

1.25000000e-03 r=3.125540e+00 m=2.323730e-03 e=2.325027e-03 BE=1.297181e-06 BE/M=5.582323e-04 t=75

$$\begin{array}{lll} \frac{R}{R_{asymp}} = 0.9986516640065255 & \frac{M}{M_{asymp}} = 0.9948865283759023 & \frac{BE}{BE_{asymp}} = 0.9922616348599246 \\ 6.25000000e-04 & r=3.127650e+00 & m=1.163057e-03 \quad e=1.163381e-03 \quad BE=3.245573e-07 \quad BE/M=2.790555e-04 \quad t=69 \\ \frac{R}{R_{asymp}} = 0.9993258535106289 & \frac{M}{M_{asymp}} = 0.9974412439490421 & \frac{BE}{BE_{asymp}} = 0.9961254545828799 \\ 3.12500000e-04 & r=3.128705e+00 & m=5.818264e-04 \quad e=5.819076e-04 \quad BE=8.117210e-08 \quad BE/M=1.395126e-04 \quad t=67 \\ \frac{R}{R_{asymp}} = 0.9996629321113595 & \frac{M}{M_{asymp}} = 0.9987201166989614 & \frac{BE}{BE_{asymp}} = 0.9980613854222472 \\ 1.56250000e-04 & r=3.129232e+00 & m=2.909877e-04 \quad e=2.910080e-04 \quad BE=2.029712e-08 \quad BE/M=6.975250e-05 \quad t=67 \\ \frac{R}{R_{asymp}} = 0.9998314673920934 & \frac{M}{M_{asymp}} = 0.9993599320035969 & \frac{BE}{BE_{asymp}} = 0.999030357099086 \\ 7.81250000e-05 & r=3.129496e+00 & m=1.455125e-04 \quad e=1.455176e-04 \quad BE=5.074792e-09 \quad BE/M=3.487530e-05 \quad t=67 \\ \frac{R}{R_{asymp}} = 0.9999157340298255 & \frac{M}{M_{asymp}} = 0.9996799344119525 & \frac{BE}{BE_{asymp}} = 0.9995150946284376 \\ 3.90625000e-05 & r=3.129628e+00 & m=7.276091e-05 \quad e=7.276218e-05 \quad BE=1.268762e-09 \quad BE/M=1.743741e-05 \quad t=66 \\ \frac{R}{R_{asymp}} = 0.9999578670983169 & \frac{M}{M_{asymp}} = 0.9998399593080929 & \frac{BE}{BE_{asymp}} = 0.9997575263316804 \\ 1.95312500e-05 & r=3.129694e+00 & m=3.638162e-05 \quad e=3.638194e-05 \quad BE=3.171985e-10 \quad BE/M=8.718648e-06 \quad t=66 \\ \frac{R}{R_{asymp}} = 0.9999789335700044 & \frac{M}{M_{asymp}} = 0.999919977679523 & \frac{BE}{BE_{asymp}} = 0.999878757919923 \\ 9.76562500e-06 & r=3.129727e+00 & m=1.819110e-05 \quad e=1.819118e-05 \quad BE=7.930063e-11 \quad BE/M=4.359309e-06 \quad t=66 \\ \frac{R}{R_{asymp}} = 0.9999894667902132 & \frac{M}{M_{asymp}} = 0.9999599883461242 & \frac{BE}{BE_{asymp}} = 0.999939377648447 \\ 4.88281250e-06 & r=3.129743e+00 & m=9.095623e-06 \quad e=9.095643e-06 \quad BE=1.982528e-11 \quad BE/M=2.179651e-06 \quad t=66 \\ \frac{R}{R_{asymp}} = 0.9999947333964092 & \frac{M}{M_{asymp}} = 0.9999799940496521 & \frac{BE}{BE_{asymp}} = 0.9999696884963407 \\ 2.44140625e-06 & r=3.129751e+00 & m=4.547830e-06 \quad e=4.547835e-06 \quad BE=4.956336e-12 \quad BE/M=1.089825e-06 \quad t=65 \\ \frac{R}{R_{asymp}} = 0.9999973666985303 & \frac{M}{M_{asymp}} = 0.9999899969939735 & \frac{BE}{BE_{asymp}} = 0.9999848441661993 \\ 1.22070312e-06 & r=3.129756e+00 & m=2.273919e-06 \quad e=2.273921e-06 \quad BE=1.239086e-12 \quad BE/M=5.449120e-07 \quad t=65 \\ \frac{R}{R_{asymp}} = 0.9999986833493466 & \frac{M}{M_{asymp}} = 0.9999949984892738 & \frac{BE}{BE_{asymp}} = 0.9999924220626071 \\ 6.10351562e-07 & r=3.129758e+00 & m=1.136961e-06 \quad e=1.136961e-06 \quad BE=3.097718e-13 \quad BE/M=2.724560e-07 \quad t=65 \\ \frac{R}{R_{asymp}} = 0.9999993416746935 & \frac{M}{M_{asymp}} = 0.9999974992427088 & \frac{BE}{BE_{asymp}} = 0.9999962110261806 \\ 3.05175781e-07 & r=3.129759e+00 & m=5.684807e-07 \quad e=5.684808e-07 \quad BE=7.744297e-14 \quad BE/M=1.362280e-07 \quad t=64 \\ \frac{R}{R_{asymp}} = 0.9999996708373515 & \frac{M}{M_{asymp}} = 0.9999987496208727 & \frac{BE}{BE_{asymp}} = 0.99999810551181 \end{array}$$

mp.dps =20    mp decimal precision =21    sage decimal precision =24

The star at  $\rho(0) = \rho_{EW}$

In [39]:

```
star_data_EW = coreless_star_set[0][skey(0.5)][ 'data' ]
mass_EW = myR(star_data_EW[ 'mass' ])
radius_EW = myR(star_data_EW[ 'radius' ])
EW = (mass_EW, radius_EW)
EW
```

Out [39]: (0.23241956266102788692000, 1.2964405430063191045000)

The star at  $\hat{\rho}(0) = 10^8$

```
In [40]: rhohat_0_norm_BSM = mpf(1e8)/rhohat_EW_mpf
star_BSM = make_star(rhohat_0_norm_BSM)
mass_BSM = myR(star_BSM['data']['mass'])
radius_BSM = myR(star_BSM['data']['radius'])
BSM = (mass_BSM, radius_BSM)
BSM
```

Out [40]: (0.19596684210709988734000, 1.4015767144639288523000)

## Plots

collect star\_data in two dictionaries, **cored\_stars** and **coreless\_stars**

**stars** is the union of the two, a dictionary of all the stars

The star's key in these dictionaries is **central\_density** (number, not string), for sorting.

```
In [41]: cored_stars = {}
for starset in star_set:
    for star_key, star in starset.items():
        if star_key in cored_stars:
            print(star_key, ' DUPLICATE')
            star_data = star['data']
            central_density = star_data['central density']
            cored_stars[central_density] = star['data']
cored_stars = dict(sorted(cored_stars.items()))
#
coreless_stars = {}
for starset in coreless_star_set:
    for star_key, star in starset.items():
        if star_key in coreless_stars:
            print(star_key, ' DUPLICATE')
            star_data = star['data']
            central_density = star_data['central density']
            coreless_stars[central_density] = star['data']
coreless_stars = dict(sorted(coreless_stars.items()))
#
stars = coreless_stars | cored_stars
stars = dict(sorted(stars.items()))
```

```
In [42]: star_plot_joined = plots(stars, 'mass', 'radius', joined=True)
#show(star_plot_joined, ymin=0, xmin=0)
plt=star_plot_joined
#plt.set_aspect_ratio(.05)
plt.set_axes_range(xmin=0, ymin=0)
plt.axes_labels([r"$\hat{M}$", r"$\hat{R}$"])
plt_bo1=plt
plt_bo2=plt
plt_bo0=plt
plt += point(EW)
plt += text(r"$\hat{\rho}(0) = \hat{\rho}_{\mathrm{EW}}$", (mass_EW+.02, radius_EW-.05), \
            fontsize='medium')
plt.axes_labels([r"$\hat{M}$", r"$\hat{R}$"])
plt.set_aspect_ratio(.1)
show(plt, axes_labels_size=1.2)
plt.save('plots/M_R.pdf', dpi=600, axes_labels_size=1.2)
#
star_plot_unjoined = plots(stars, 'mass', 'radius', joined=False)
#show(star_plot_unjoined, ymin=0, xmin=0)
plt=star_plot_unjoined
#plt.set_aspect_ratio(.05)
plt.set_axes_range(xmin=0, ymin=0)
plt.axes_labels([r"$\hat{M}$", r"$\hat{R}$"])
plt_bo1_unj=plt
plt_bo2_unj=plt
plt_bo0_unj=plt
plt += point(EW)
plt += text(r"$\hat{\rho}(0) = \hat{\rho}_{\mathrm{EW}}$", (mass_EW+.02, radius_EW-.05), \
```

```

        fontsize='medium')
plt.axes_labels([r"$\hat{M}$",r"$\hat{R}$"])
plt.set_aspect_ratio(.1)
show(plt,axes_labels_size=1.2)

```

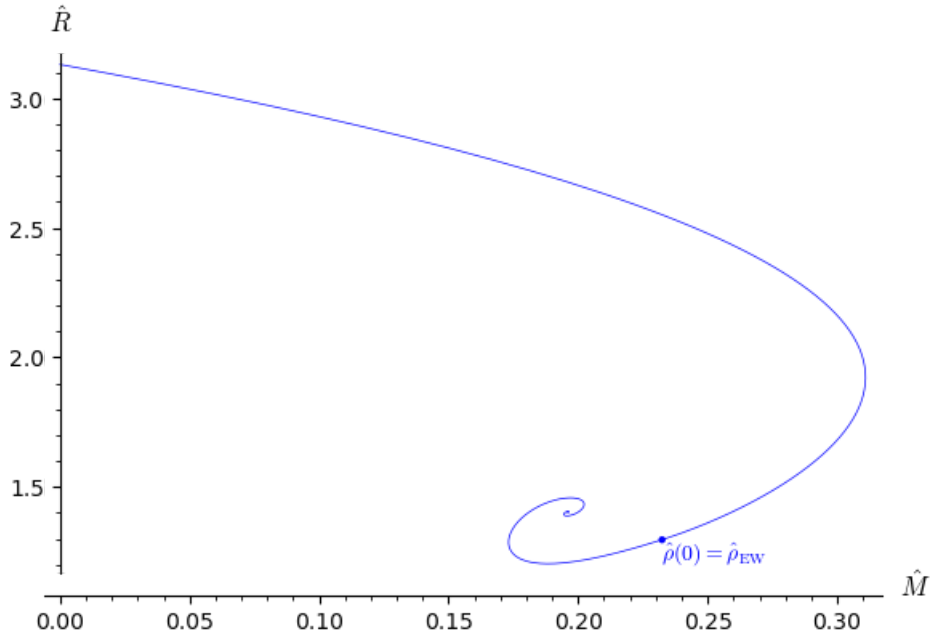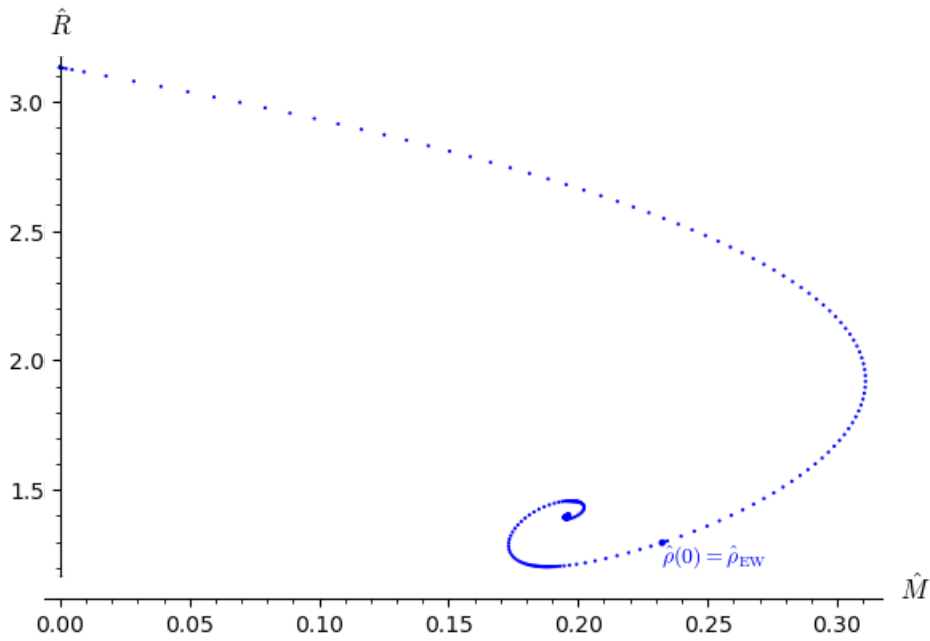

In [43]:

```

plt_bo1.set_aspect_ratio(.1)
plt_bo1.set_axes_range(xmin=0.172,xmax=.21,ymin=1.2,ymax=1.46)
show(plt_bo1,title="M R blowup 1",fontsize=13,axes_labels_size=1.2)
plt_bo1.save('plots/M_Rblowup1.pdf',dpi=600,fontsize=13,axes_labels_size=1.2)
#
plt_bo2 = plt_bo0
plt_bo2 += point(BSM)
plt_bo2 += text(r"$\hat{\rho}(0) = 10^8$", (mass_BSM-0.0003,radius_BSM-.0005),fontsize='large')
plt_bo2.set_aspect_ratio(.1)
plt_bo2.set_axes_range(xmin=0.1944,xmax=.197,ymin=1.387,ymax=1.406)
plt_bo2.axes_labels([r"$\hat{M}$",r"$\hat{R}$"])
show(plt_bo2,title="M R blowup 2",fontsize=13,axes_labels_size=1.2)
plt_bo2.save('plots/M_Rblowup2.pdf',dpi=600,fontsize=13,axes_labels_size=1.2)
#
plt_bo1_unj.set_aspect_ratio(.1)
plt_bo1_unj.set_axes_range(xmin=0.172,xmax=.21,ymin=1.2,ymax=1.46)
show(plt_bo1_unj,title="M R blowup 1",fontsize=13,axes_labels_size=1.2)
#
plt_bo2_unj = plt_bo0_unj
plt_bo2_unj += point(BSM)
plt_bo2_unj += text(r"$\hat{\rho}(0) = 10^8$", (mass_BSM-0.0003,radius_BSM-.0005),fontsize='large')
plt_bo2_unj.set_aspect_ratio(.1)

```

```
plt_bo2_unj.set_axes_range(xmin=0.1944,xmax=.197,ymin=1.387,ymax=1.406)
plt_bo2_unj.axes_labels([r"$\hat{M}$",r"$\hat{R}$"])
show(plt_bo2_unj,title="M R blowup 2",fontsize=13,axes_labels_size=1.2)
```

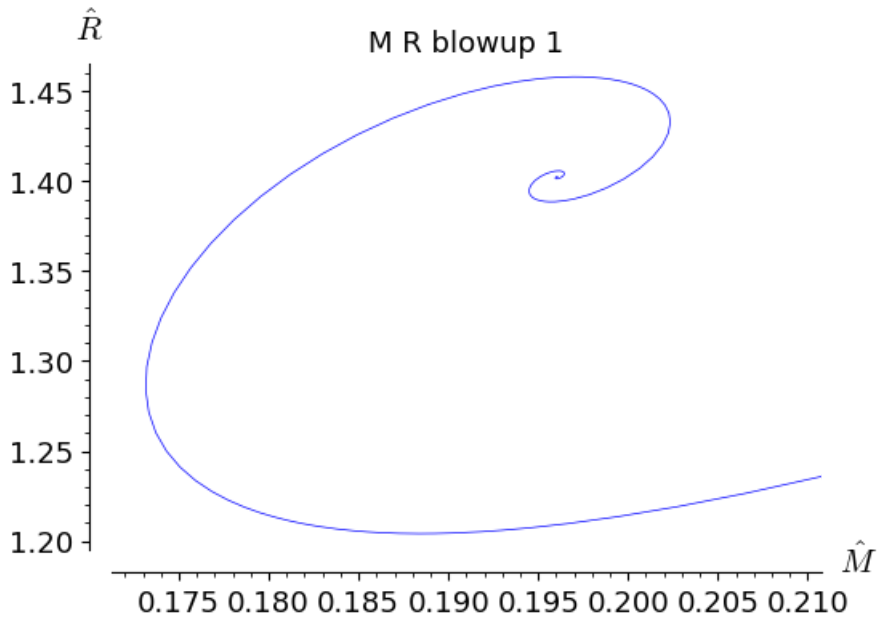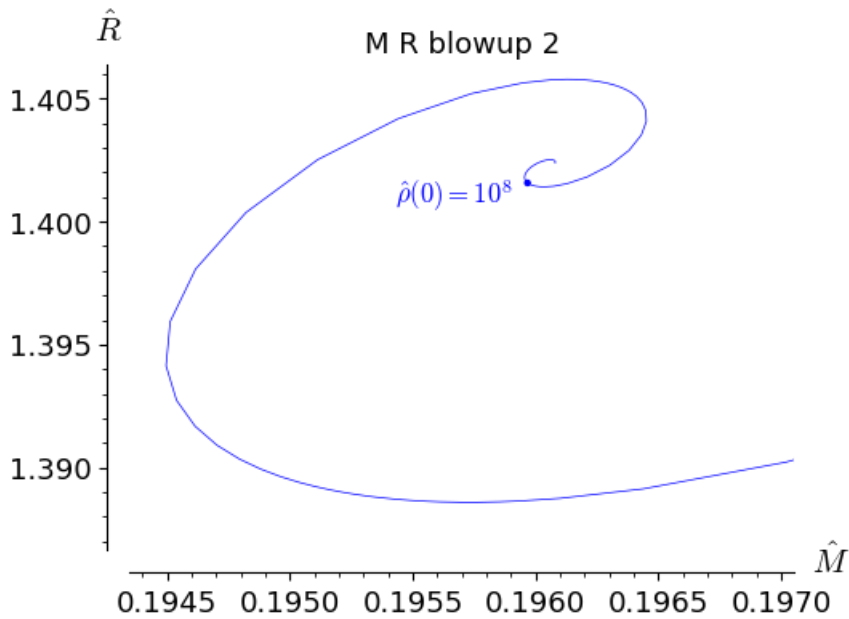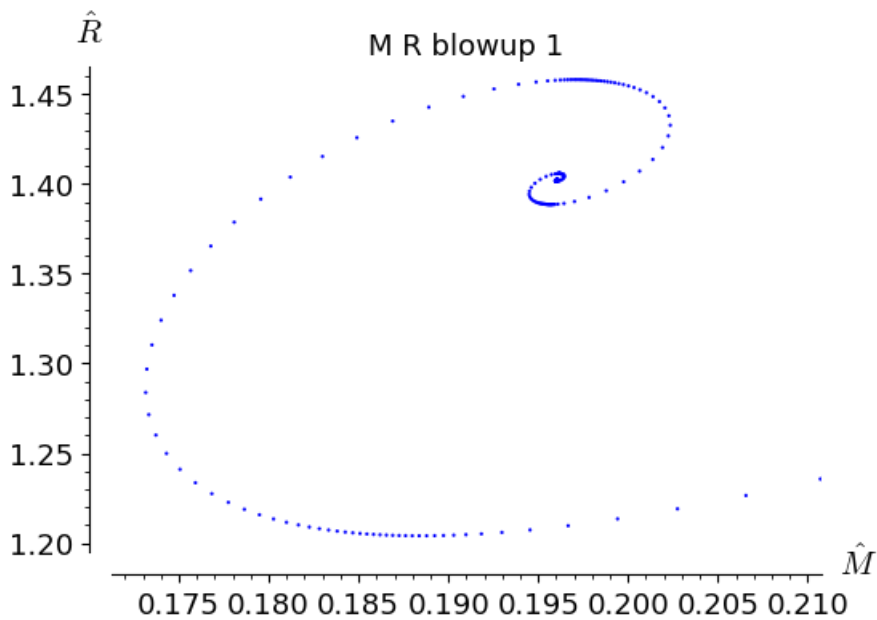

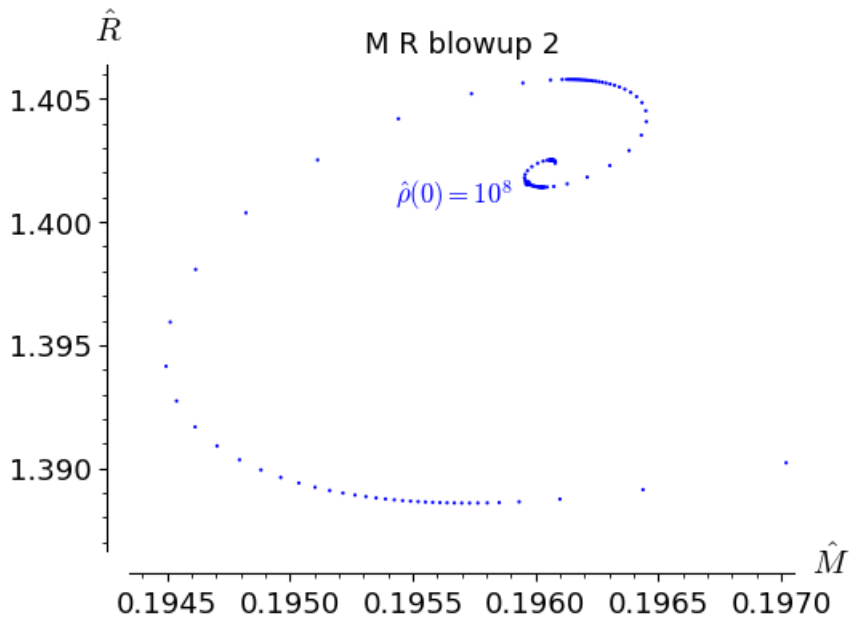

In [44]:

```
BElist = []
for central_density, star_data in stars.items():
    mass = star_data['mass']
    energy = star_data['energy']
    BE = energy - mass
    BE_ratio = (energy - mass) / mass
    BElist.append([mass, -BE])
plt = list_plot(BElist, marker=None, plotjoined=True, thickness=0.5)
# plt.set_axes_range(xmin=0, ymin=0)
plt.axes_labels([r"$\hat{M}$", r"$-\hat{BE}$"])
show(plt, fontsize=13, axes_labels_size=1.2)
plt.save('plots/M_BE.pdf', dpi=600, fontsize=13, axes_labels_size=1.2)
#
BEratiolist = []
for central_density, star_data in stars.items():
    mass = star_data['mass']
    energy = star_data['energy']
    BE_ratio = (energy - mass) / mass
    BEratiolist.append([mass, -BE_ratio])
plt = list_plot(BEratiolist, marker=None, plotjoined=True, thickness=0.5)
# plt.set_axes_range(xmin=0, ymin=0)
plt.axes_labels([r"$\hat{M}$", r"$-\hat{BE}/\hat{M}$"])
show(plt, fontsize=13, axes_labels_size=1.2)
plt.save('plots/M_BEratio.pdf', dpi=600, fontsize=13, axes_labels_size=1.2)
```

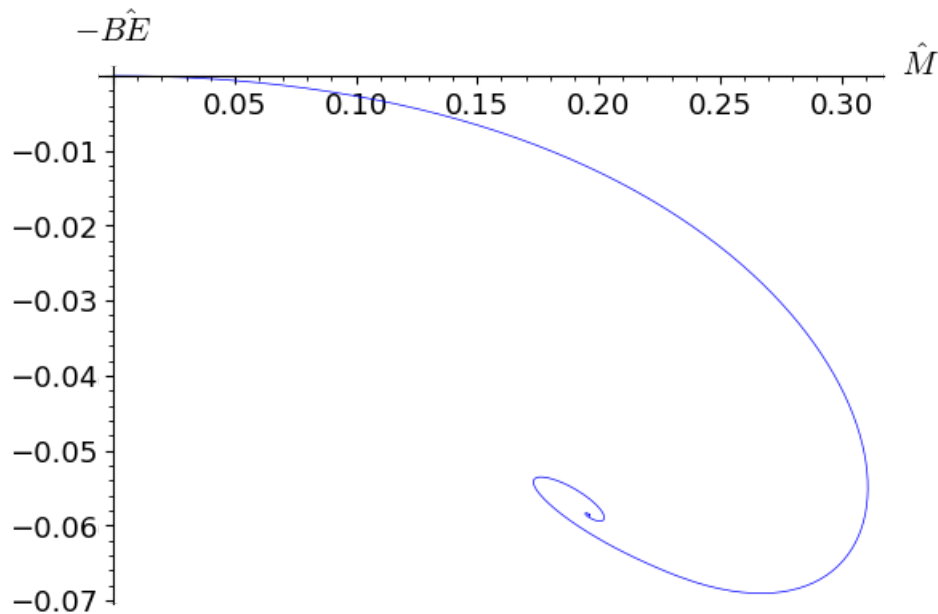

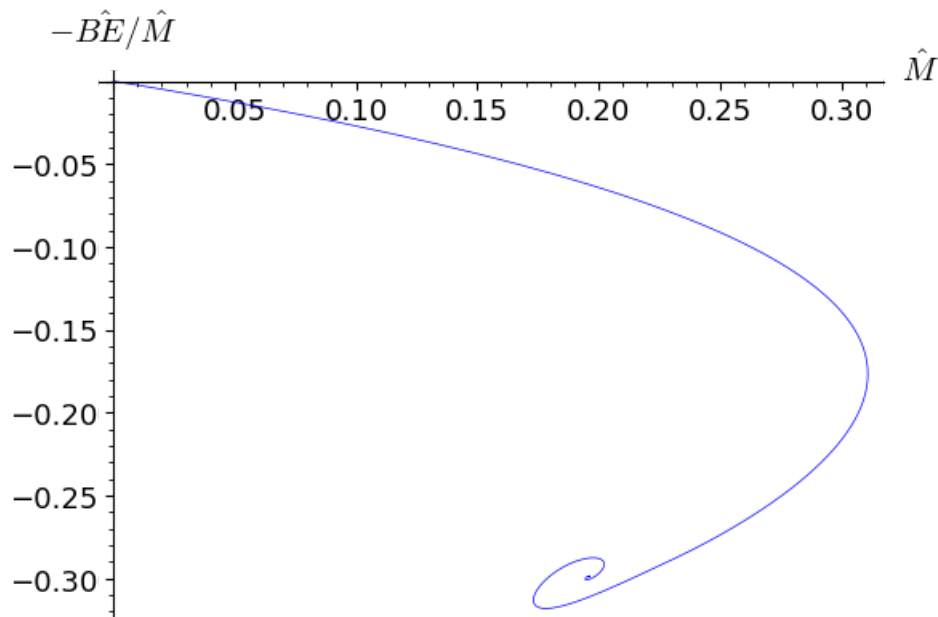

## Special stars

The star of minimum radius.

3.20219250e+00 r=1.204027e+00 m=1.883777e-01 e=2.477540e-01 BE=5.937627e-02 BE/M=3.151979e-01 t=6

```
In [45]: star_data_min_R = star_set[1]['3.20219250e+00']['data']
mass_min_R = myR(star_data_min_R['mass'])
radius_min_R = myR(star_data_min_R['radius'])
min_R = (mass_min_R, radius_min_R)
min_R
```

```
Out[45]: (0.18837772352835232517000, 1.2040273735813345141000)
```

The star of largest mass

3.47709480e-01 r=1.896051e+00 m=3.108239e-01 e=3.670901e-01 BE=5.626628e-02 BE/M=1.810230e-01 t=12

3.41803251e-01 r=1.918823e+00 m=3.109591e-01 e=3.661058e-01 BE=5.514674e-02 BE/M=1.773441e-01 t=12

3.35874144e-01 r=1.941588e+00 m=3.108993e-01 e=3.648964e-01 BE=5.399716e-02 BE/M=1.736805e-01 t=12

```
In [46]: for star_key in ['3.47709480e-01', '3.41803251e-01', '3.35874144e-01']:
print(coreless_star_set[1][star_key]['ode']['initial value'])
```

```
0.34770947997778476825
0.34180325054452595958
0.335874143802153429
```

```
In [47]: star_set_search_largest_m={}
for x in srangle(0.336,0.347,.001,universe=RDF):
x=Reals(round(x,4))
star = make_coreless_star(x)
star_data = star['data']
star_key = star['star key']
print_star(star_key,star_data)
star_set_search_largest_m[star_key]=star
```

```
3.36000000e-01 r=1.941106e+00 m=3.109026e-01 e=3.649244e-01 BE=5.402181e-02 BE/M=1.737580e-01 t=0
3.37000000e-01 r=1.937273e+00 m=3.109256e-01 e=3.651430e-01 BE=5.421733e-02 BE/M=1.743739e-01 t=0
3.38000000e-01 r=1.933436e+00 m=3.109431e-01 e=3.653553e-01 BE=5.441216e-02 BE/M=1.749907e-01 t=0
3.39000000e-01 r=1.929598e+00 m=3.109551e-01 e=3.655614e-01 BE=5.460630e-02 BE/M=1.756083e-01 t=0
3.40000000e-01 r=1.925756e+00 m=3.109615e-01 e=3.657613e-01 BE=5.479974e-02 BE/M=1.762267e-01 t=0
3.41000000e-01 r=1.921912e+00 m=3.109624e-01 e=3.659549e-01 BE=5.499246e-02 BE/M=1.768460e-01 t=0
3.42000000e-01 r=1.918065e+00 m=3.109577e-01 e=3.661422e-01 BE=5.518446e-02 BE/M=1.774661e-01 t=0
3.43000000e-01 r=1.914216e+00 m=3.109474e-01 e=3.663231e-01 BE=5.537572e-02 BE/M=1.780871e-01 t=0
3.44000000e-01 r=1.910364e+00 m=3.109316e-01 e=3.664978e-01 BE=5.556624e-02 BE/M=1.787089e-01 t=0
3.45000000e-01 r=1.906509e+00 m=3.109101e-01 e=3.666661e-01 BE=5.575601e-02 BE/M=1.793316e-01 t=0
3.46000000e-01 r=1.902652e+00 m=3.108831e-01 e=3.668281e-01 BE=5.594500e-02 BE/M=1.799551e-01 t=0
```



In [48]:

```
star = star_set_search_largest_m['3.41000000e-01']
star_data = star['data']
mass = Reals(star_data['mass'])
radius = Reals(star_data['radius'])
energy = Reals(star_data['energy'])
BE = energy-mass
pretty_print(LE(r"\hat M = "),mass,LE(r"\qqquad M = "),mass*m_b_kg,LE(r" = "),mass*m_b_solar,LE(r"M_\odot"))
pretty_print(LE(r"\hat R = "),radius,LE(r"\qqquad R = "),radius*r_b_m)
pretty_print(LE(r"\frac{BE}{M} = "),BE/mass)
```

$$\hat{M} = 0.31096240159359108330000 \quad M = 1.8183901269497294 \times 10^{25} \text{ kg} = 9.14499158594714 \times 10^{-06} M_{\odot}$$

$$\hat{R} = 1.9219122503640596194000 \quad R = 0.08345974544494067 \text{ m}$$

$$\frac{BE}{M} = 0.17684600815657502834582$$

## The mass where transitions become possible

9.23643135e+00 r=1.271494e+00 m=1.733260e-01 e=2.278757e-01 BE=5.454964e-02 BE/M=3.147227e-01 t=6

1.02705121e+01 r=1.283822e+00 m=1.731541e-01 e=2.274269e-01 BE=5.427287e-02 BE/M=3.134369e-01 t=6

1.14397938e+01 r=1.296846e+00 m=1.732126e-01 e=2.272499e-01 BE=5.403726e-02 BE/M=3.119707e-01 t=6

In [49]:

```
star_set_search_transition={}
for x in srange(9.24,11.43,.2,universe=RDF):
    x=Reals(round(x,4))
    star = make_star(x)
    star_data = star['data']
    star_key = star['star key']
    print_star(star_key,star_data)
    star_set_search_transition[star_key]=star
```

```
9.24000000e+00 r=1.271538e+00 m=1.733250e-01 e=2.278735e-01 BE=5.454855e-02 BE/M=3.147183e-01 t=0
9.44000000e+00 r=1.273979e+00 m=1.732717e-01 e=2.277609e-01 BE=5.448919e-02 BE/M=3.144725e-01 t=0
9.64000000e+00 r=1.276393e+00 m=1.732288e-01 e=2.276616e-01 BE=5.443281e-02 BE/M=3.142249e-01 t=0
9.84000000e+00 r=1.278779e+00 m=1.731956e-01 e=2.275748e-01 BE=5.437924e-02 BE/M=3.139759e-01 t=0
1.00400000e+01 r=1.281138e+00 m=1.731714e-01 e=2.274998e-01 BE=5.432836e-02 BE/M=3.137259e-01 t=0
1.02400000e+01 r=1.283469e+00 m=1.731558e-01 e=2.274358e-01 BE=5.428003e-02 BE/M=3.134752e-01 t=0
1.04400000e+01 r=1.285771e+00 m=1.731480e-01 e=2.273822e-01 BE=5.423413e-02 BE/M=3.132240e-01 t=0
1.06400000e+01 r=1.288044e+00 m=1.731478e-01 e=2.273384e-01 BE=5.419054e-02 BE/M=3.129727e-01 t=0
1.08400000e+01 r=1.290289e+00 m=1.731546e-01 e=2.273037e-01 BE=5.414916e-02 BE/M=3.127215e-01 t=0
1.10400000e+01 r=1.292504e+00 m=1.731679e-01 e=2.272778e-01 BE=5.410987e-02 BE/M=3.124706e-01 t=0
1.12400000e+01 r=1.294691e+00 m=1.731874e-01 e=2.272600e-01 BE=5.407259e-02 BE/M=3.122201e-01 t=0
```

In [50]:

```
star = star_set_search_transition['1.06400000e+01']
star_data = star['data']
mass = Reals(star_data['mass'])
radius = Reals(star_data['radius'])
energy = Reals(star_data['energy'])
BE = energy-mass
pretty_print(LE(r"\hat M = "),mass,LE(r"\qqquad M = "),mass*m_b_kg,LE(r" = "),mass*m_b_solar,LE(r"M_\odot"))
pretty_print(LE(r"\hat R = "),radius,LE(r"\qqquad R = "),radius*r_b_m)
pretty_print(LE(r"\frac{BE}{M} = "),BE/mass)
```

$$\hat{M} = 0.17314781111503715215000 \quad M = 1.0125026968566777 \times 10^{25} \text{ kg} = 5.092047358965388 \times 10^{-06} M_{\odot}$$

$$\hat{R} = 1.2880442749896468792000 \quad R = 0.05593379577662084 \text{ m}$$

$$\frac{BE}{M} = 0.31297271924251858054214$$

## The star of largest BE/M

In [51]:

```
star_set_search={}
for x in srange(5.21,5.30,.01,universe=RDF):
    x=Reals(round(x,4))
    star = make_star(x)
```

```

star_data = star['data']
star_key = star['star key']
print_star(star_key,star_data)
star_set_search[star_key]=star

```

```

5.21000000e+00 r=1.219663e+00 m=1.784181e-01 e=2.351704e-01 BE=5.675226e-02 BE/M=3.180858e-01 t=0
5.22000000e+00 r=1.219782e+00 m=1.783891e-01 e=2.351322e-01 BE=5.674309e-02 BE/M=3.180861e-01 t=0
5.23000000e+00 r=1.219902e+00 m=1.783602e-01 e=2.350941e-01 BE=5.673395e-02 BE/M=3.180864e-01 t=0
5.24000000e+00 r=1.220022e+00 m=1.783314e-01 e=2.350563e-01 BE=5.672484e-02 BE/M=3.180866e-01 t=0
5.25000000e+00 r=1.220142e+00 m=1.783028e-01 e=2.350186e-01 BE=5.671576e-02 BE/M=3.180867e-01 t=0
5.26000000e+00 r=1.220262e+00 m=1.782743e-01 e=2.349810e-01 BE=5.670670e-02 BE/M=3.180868e-01 t=0
5.27000000e+00 r=1.220383e+00 m=1.782460e-01 e=2.349436e-01 BE=5.669767e-02 BE/M=3.180867e-01 t=0
5.28000000e+00 r=1.220503e+00 m=1.782177e-01 e=2.349064e-01 BE=5.668867e-02 BE/M=3.180866e-01 t=0
5.29000000e+00 r=1.220624e+00 m=1.781896e-01 e=2.348693e-01 BE=5.667970e-02 BE/M=3.180864e-01 t=0

```

In [52]:

```

star = star_set_search['5.26000000e+00']
star_data = star['data']
mass = Reals(star_data['mass'])
radius = Reals(star_data['radius'])
energy = Reals(star_data['energy'])
BE = energy-mass
pretty_print(LE(r"\hat M = "),mass,LE(r"\qqquad M = "),mass*m_b_kg,LE(r" = "),mass*m_b_solar,LE(r"M_\infty"))
pretty_print(LE(r"\hat R = "),radius,LE(r"\qqquad R = "),radius*r_b_m)
pretty_print(LE(r"\frac{BE}{M} = "),BE/mass)

```

$$\hat{M} = 0.17827431985146075410000 \quad M = 1.0424805746459594 \times 10^{25} \text{ kg} = 5.24281117806256 \times 10^{-06} M_{\odot}$$

$$\hat{R} = 1.2202620922647479658000 \quad R = 0.05299032959347387 \text{ m}$$

$$\frac{BE}{M} = 0.31808676121034497896813$$

## Not used in the paper

### radius / Schwarzschild radius

In [53]:

```

Rratiolist = []
for central_density,star_data in stars.items():
    mass = star_data['mass']
    radius = star_data['radius']
    Rratiolist.append([mass,radius/(2*mass)])
plt = list_plot(Rratiolist,marker=None,plotjoined=True,thickness=0.5)

```

In [54]:

```

plt.set_axes_range(xmin=0,xmax=0.32)
plt.axes_labels([r"$\hat M$",r"$\frac{R}{r_s}$"])
show(plt,fontsize=13,axes_labels_size=1.2,scale="semilogy")
#plt.save('plots/M_BEratio.pdf',dpi=600,fontsize=13,axes_labels_size=1.2)

```

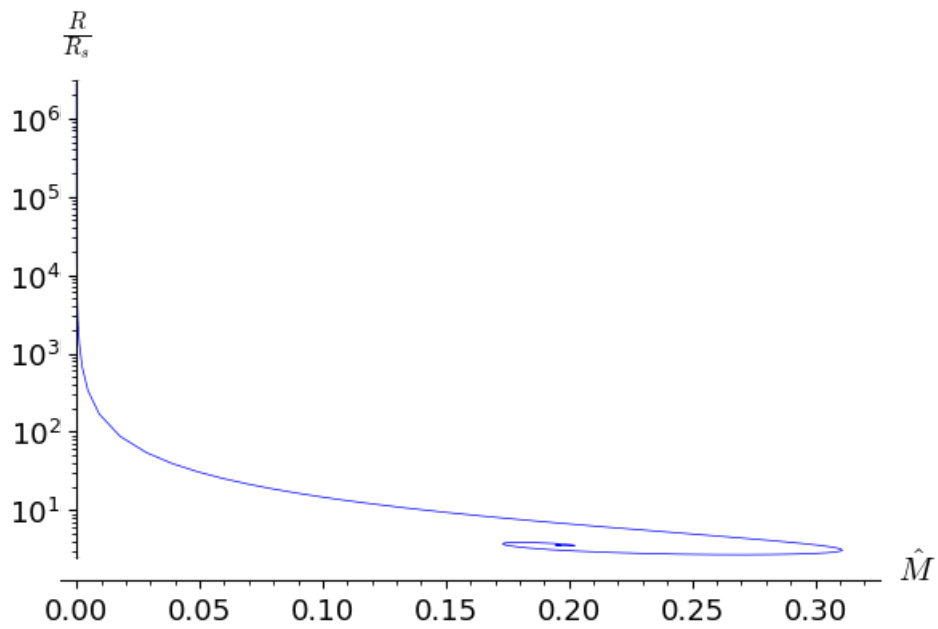

```
In [55]: plt.set_axes_range(xmin=0,xmax=0.32,ymax=3)
plt.axes_labels([r"$\hat{M}$",r"$\frac{R}{R_s}$"])
show(plt,fontsize=13,axes_labels_size=1.2)
```

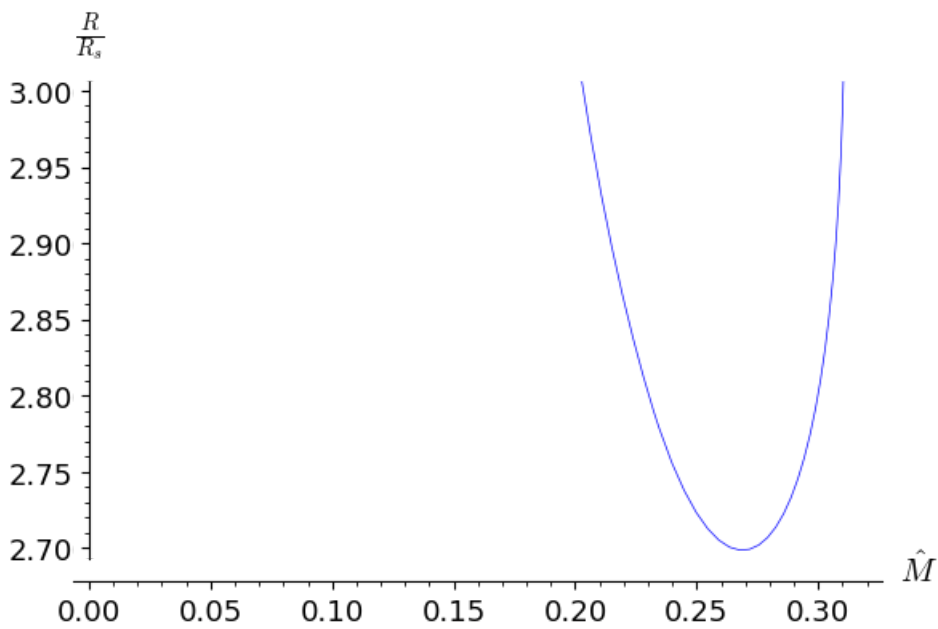

```
In [56]: plt.set_axes_range(xmin=0.05,xmax=0.15,ymin=10,ymax=20)
plt.axes_labels([r"$\hat{M}$",r"$\frac{R}{R_s}$"])
show(plt,fontsize=13,axes_labels_size=1.2)
```

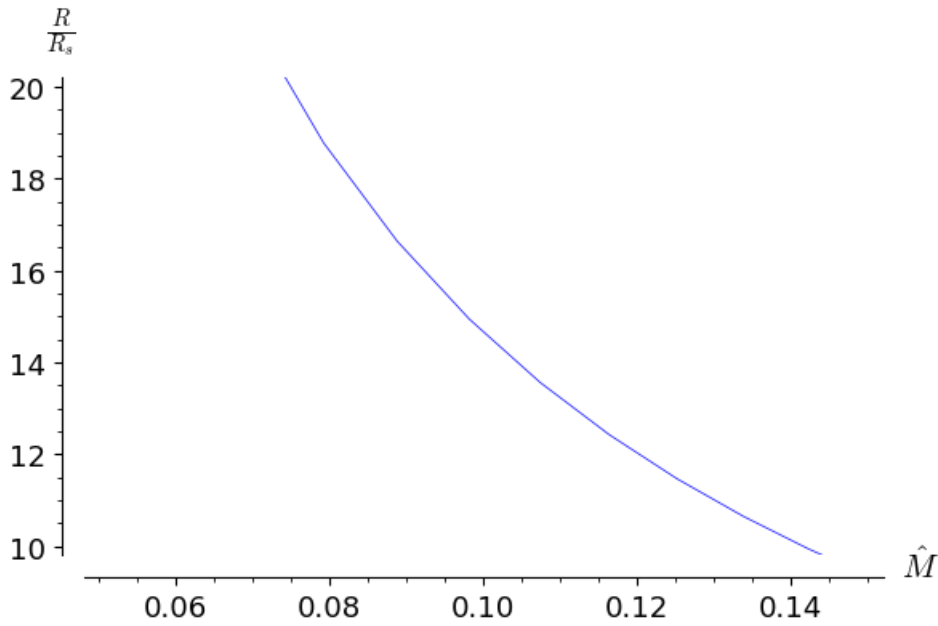

Core radius / radius and core mass / mass

In [57]:

```
core_radius_ratios = []
for central_density, star_data in cored_stars.items():
    mass = star_data['mass']
    core_radius_ratio = star_data['core radius']/star_data['radius']
    core_radius_ratios.append([mass, core_radius_ratio])
#list_plot(core_radius_ratios, marker='.', size=10)
plt = list_plot(core_radius_ratios, marker=None, plotjoined=True, thickness=0.5)
#plt.set_axes_range(xmin=0, ymin=0)
plt.axes_labels([r"$\hat{M}$", r"$\hat{R}_{\mathrm{core}}/\hat{R}$"])
show(plt, title="Rcore/R", fontsize=13, axes_labels_size=1.2)
plt.save('plots/M_Rcoreratio.pdf', dpi=600, fontsize=13, axes_labels_size=1.2)
#
core_mass_ratios = []
for central_density, star_data in cored_stars.items():
    mass = star_data['mass']
    core_mass_ratio = star_data['core mass']/star_data['mass']
    core_mass_ratios.append([mass, core_mass_ratio])
plt = list_plot(core_mass_ratios, marker=None, plotjoined=True, thickness=0.5)
plt.axes_labels([r"$\hat{M}$", r"$\hat{M}_{\mathrm{core}}/\hat{M}$"])
show(plt, title="Mcore/M", fontsize=13, axes_labels_size=1.2)
plt.save('plots/M_Mcoreratio.pdf', dpi=600, fontsize=13, axes_labels_size=1.2)
#list_plot(core_mass_ratios, marker='.', size=10)
```

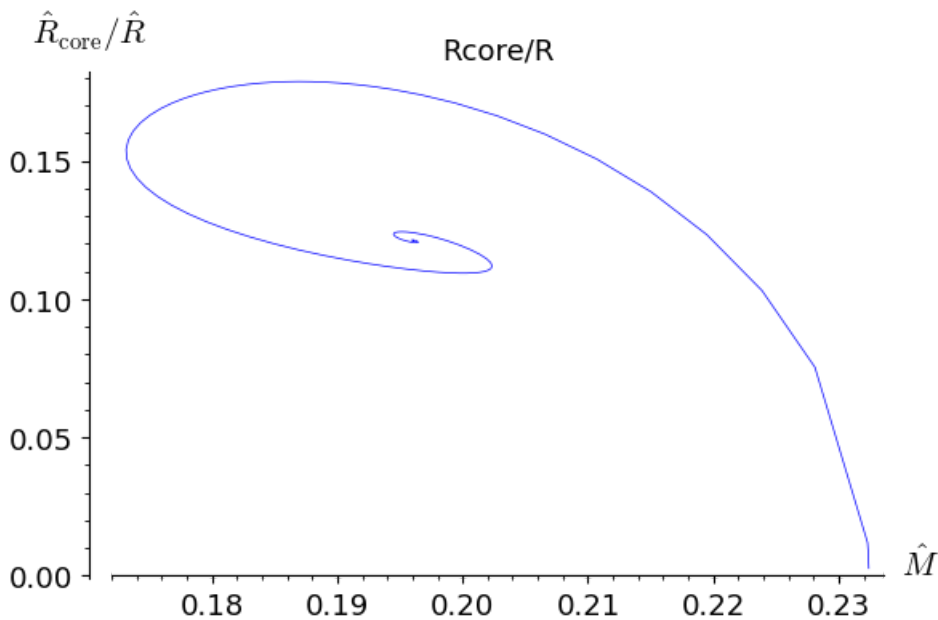

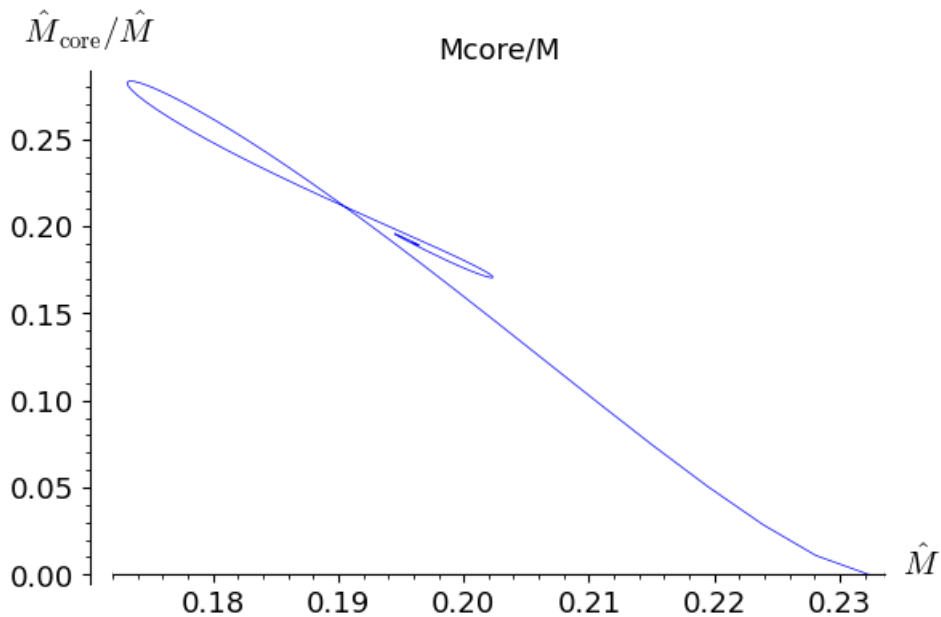

mass profile of a cloud

In [58]:

```
set_precision(30)
star = make_coreless_star(3.0517578125e-7, return_ode=True)
ode = star['ode']
star_data = star['data']
shell_ode = ode['shell ode']
initial_value = ode['initial value']
mass = star_data['mass']
#
r_fun = lambda m: Reals(shell_ode(m)[0])
m_fun = lambda m: Reals(shell_ode(m)[1]/mass)
plt = parametric_plot((r_fun, m_fun), (m, 0, initial_value))
#
set_precision()
#
plt.set_aspect_ratio(2)
plt.axes_labels([r"$\hat{r}$", r"$\hat{m}/\hat{M}$"])
show(plt, fontsize=13, axes_labels_size=1.2)
```

mp.dps =30    mp decimal precision =31    sage decimal precision =34

mp.dps =20    mp decimal precision =21    sage decimal precision =24

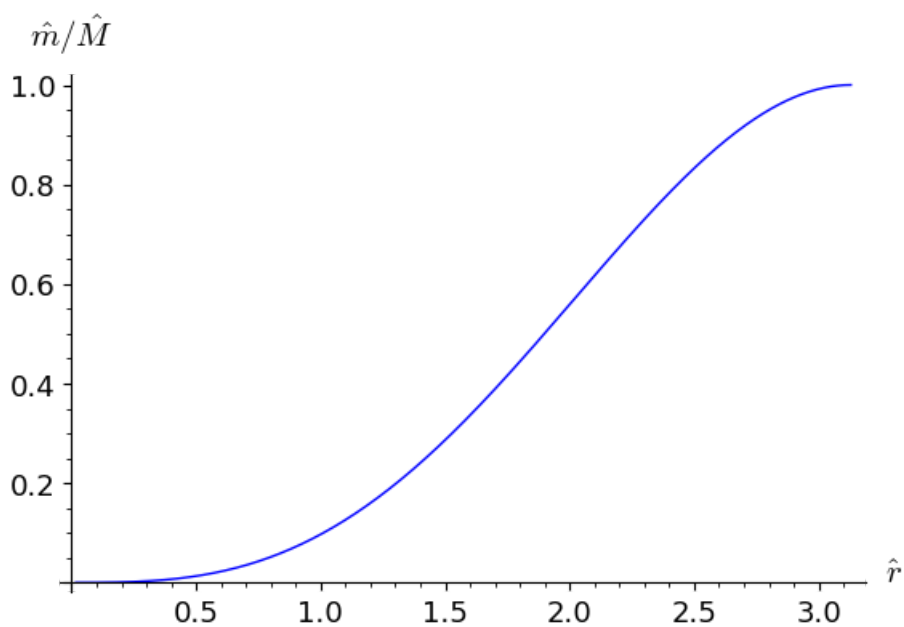

mass profiles of massive stars

3 stars of same mass, different radius and binding energy

1.19892328e-01 r=2.721241e+00 m=1.812195e-01 e=1.913617e-01 BE=1.014224e-02 BE/M=5.596662e-02 t=12  
2.86784664e+01 r=1.403815e+00 m=1.812014e-01 e=2.350428e-01 BE=5.384138e-02 BE/M=2.971356e-01 t=6  
4.47166984e+00 r=1.211533e+00 m=1.809907e-01 e=2.385063e-01 BE=5.751560e-02 BE/M=3.177822e-01 t=6

In [59]:

```
star_key1 = '1.19892328e-01'
star1 = coreless_star_set[1][star_key1]
star_key2 = '2.86784664e+01'
star2 = star_set[1][star_key2]
star_key3 = '4.47166984e+00'
star3 = star_set[1][star_key3]
print(star1['ode']['initial value'])
print(star2['ode']['initial value'])
print(star3['ode']['initial value'])
```

```
0.11989232813047308982
28.678466396330248299
4.4716698404048722934
```

In [60]:

```
star1 = make_coreless_star(0.11989232813047308982,return_ode=True)
star2 = make_star(28.678466396330248299,return_ode=True)
star3 = make_star(4.4716698404048722934,return_ode=True)
star_key1 = '1.19892328e-01'
star_key2 = '2.86784664e+01'
star_key3 = '4.47166984e+00'

star_key = star_key1
star = star1
ode = star['ode']
star_data = star['data']
shell_ode = ode['shell ode']
initial_value = ode['initial value']
mass = star_data['mass']
#
r_fun = lambda m: Reals(shell_ode(m)[0])
m_fun = lambda m: Reals(shell_ode(m)[1]/mass)
plt1 = parametric_plot((r_fun,m_fun),(m,0,initial_value))
#
plt1.set_aspect_ratio(2)
plt1.axes_labels([r"$\hat{r}$",r"$\hat{m}/\hat{M}$"])
#show(plt,fontsize=13,axes_labels_size=1.2)

star_key = star_key2
star = star2
ode = star['ode']
star_data = star['data']
shell_ode = ode['shell ode']
core_ode = ode['core ode']
initial_value = ode['initial value']
mass = star_data['mass']
#
rhoh = var('rhoh')
core_r = lambda rhoh: Reals(core_ode(rhoh)[0])
core_m = lambda rhoh: Reals(core_ode(rhoh)[1]/mass)
bdry = core_ode(1)
r_bdry = Reals(bdry[0])
m_bdry = Reals(bdry[1]/mass)
plt_core = parametric_plot((core_r,core_m),(rhoh,1,initial_value))
plt_core += line([(r_bdry,m_bdry-.1),(r_bdry,m_bdry+.1)],linestyle=":")
#show(plt_core)
#
r_fun = lambda m: Reals(shell_ode(m)[0])
m_fun = lambda m: Reals(shell_ode(m)[1]/mass)
plt = parametric_plot((r_fun,m_fun),(m,0,0.5))
plt2 = plt+plt_core
#
plt2.set_aspect_ratio(2)
plt2.axes_labels([r"$\hat{r}$",r"$\hat{m}/\hat{M}$"])
#show(plt2,fontsize=13,axes_labels_size=1.2)

star_key = star_key3
star = star3
ode = star['ode']
star_data = star['data']
shell_ode = ode['shell ode']
core_ode = ode['core ode']
initial_value = ode['initial value']
```

```

mass = star_data['mass']
#
rho_h = var('rho_h')
core_r = lambda rho_h: Reals(core_ode(rho_h)[0])
core_m = lambda rho_h: Reals(core_ode(rho_h)[1]/mass)
bdry = core_ode(1)
r_bdry = Reals(bdry[0])
m_bdry = Reals(bdry[1]/mass)
plt_core = parametric_plot((core_r,core_m),(rho_h,1,initial_value))
plt_core += line([(r_bdry,m_bdry-.1),(r_bdry,m_bdry+.1)],linestyle=":")
#show(plt_core)
#
r_fun = lambda m: Reals(shell_ode(m)[0])
m_fun = lambda m: Reals(shell_ode(m)[1]/mass)
plt = parametric_plot((r_fun,m_fun),(m,0,0.5))
plt3 = plt+plt_core
#
plt3.set_aspect_ratio(2)
plt3.axes_labels([r"$\hat{r}$",r"$\hat{m}/\hat{M}$"])
#show(plt3,fontsize=13,axes_labels_size=1.2)

show(plt1+plt2+plt3,fontsize=13,axes_labels_size=1.2)

```

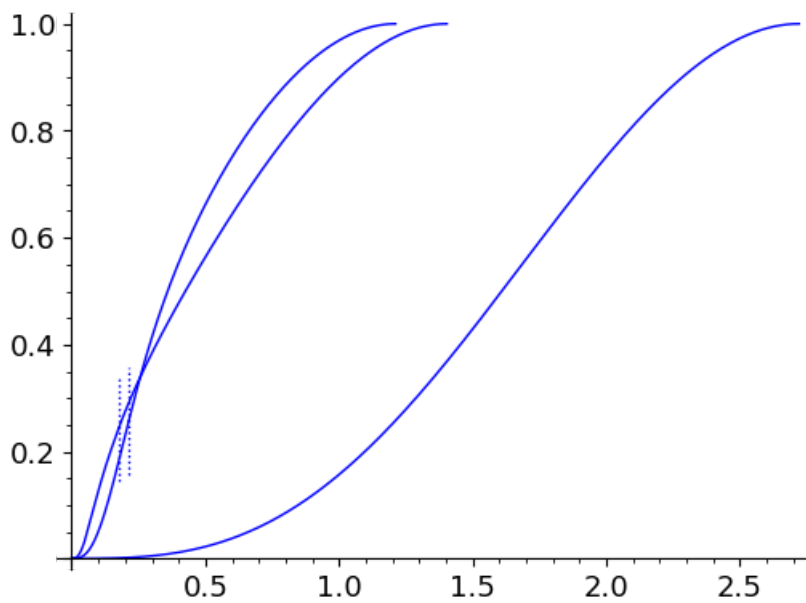

In [ ]:
