# Supplementary material for: Dark matter stars
Source: arXiv:2203.12181 ancillary file (2022-03-24)
Supplement: Supplementary file 2 [file Pure_radiation_stars.pdf]

# Pure radiation stars ( $w = 1/3$ )

(Some of this is probably in the literature.)

## Preamble

```
In [1]: %display latex
LE = lambda latex_string: LatexExpr(latex_string);
```

```
In [2]: from timeit import default_timer as timer
start=timer()
end=timer()
```

```
In [3]: from mpmath import mp
from mpmath import mpf,mpc
import sage.libs.mpmath.all as a
mp.pretty = True
```

```
In [4]: def set_precision(decimal_precision=20):
    global RealNumber,Reals,myR,sage_binary_precision,sage_decimal_precision
    mp.dps = decimal_precision
    binary_precision=mp.prec
    sage_binary_precision=mp.prec+10
    sage_decimal_precision = floor(sage_binary_precision/log(10,2))
    Reals = RealField(sage_binary_precision)
    RealNumber = Reals
    myR = Reals
    pretty_print("mp.dps = ",mp.dps,"    mp decimal precision = ", floor(mp.prec/log(10,2)),\
                "    sage decimal precision = ", sage_decimal_precision )
    set_precision(decimal_precision=20)
```

mp.dps =20      mp decimal precision =21      sage decimal precision =24

## TOV equations for a perfect fluid with constant $w$

The equation of state is

$$p = w\rho$$

with  $w$  constant. Change variables:

$$x = 4\pi Gr^2\rho \quad y = \frac{Gm}{r}$$

The TOV equations for  $m$  and  $p$  become

$$r \frac{dx}{dr} = 2x \frac{1 - (2+c)y - cw x}{1 - 2y} \quad r \frac{dy}{dr} = x - y \quad c = \frac{1}{2} \left( 1 + \frac{1}{w} \right)$$

The right hand sides are independent of  $t$ . The TOV equations are the flow equations for a vector field in the  $x, y$  plane.

## The fixed point

There is a fixed point at

$$x_\infty = y_\infty = \frac{2w}{w^2 + 6w + 1}$$

The linearized flow near the fixed point is

$$x = x_\infty + \delta x \quad y = y_\infty + \delta y$$
$$r \frac{d}{dr} \begin{pmatrix} \delta x \\ \delta y \end{pmatrix} = -A \begin{pmatrix} \delta x \\ \delta y \end{pmatrix} \quad A = \begin{pmatrix} a & b \\ -1 & 1 \end{pmatrix} \quad a = \frac{2w}{1+w} \quad b = \frac{1+5w}{(1+w)^2}$$

The eigenvalues of  $A$  are

$$\lambda_{\pm} = \frac{1 + 3w \pm i\sqrt{3 + 22w - w^2}}{2(1 + w)}$$

For  $w = \frac{1}{3}$

$$A = \begin{pmatrix} \frac{1}{2} & \frac{3}{2} \\ -1 & 1 \end{pmatrix} \quad \lambda_{\pm} = \frac{3 \pm i\sqrt{23}}{4}$$

The fixed point is attractive. The flow spirals inwards.

## Phase portrait

A plot of the flowlines, followed by two blowups.

The plot shows only direction. The flow vector is normalized to constant length.

In [5]:

```
x,y,w = var('x,y,w')
w= 1/3
vx = x*(2-(1+1/w)*(y+w*x)/(1-2*y))
vy = x-y
vnorm = sqrt(vx^2+vy^2)
vxhat = vx/vnorm
vyhat = vy/vnorm
#
plt=plot_vector_field((vxhat,vyhat),(x,0,1),(y,0,1))
#plt.set_axes_range(ymin=0)
plt.axes_labels([r"$x$",r"$y$"])
show(plt,title="Figure 1")
#plt.save('Figure_1_vf.pdf',title="Figure 1", dpi=300)
#
plt=plot_vector_field((vxhat,vyhat),(x,0,.5),(y,0,.5))
show(plt)
#
vfplot=plot_vector_field((vxhat,vyhat),(x,0,0.4),(y,0,.3))
show(vfplot)
```

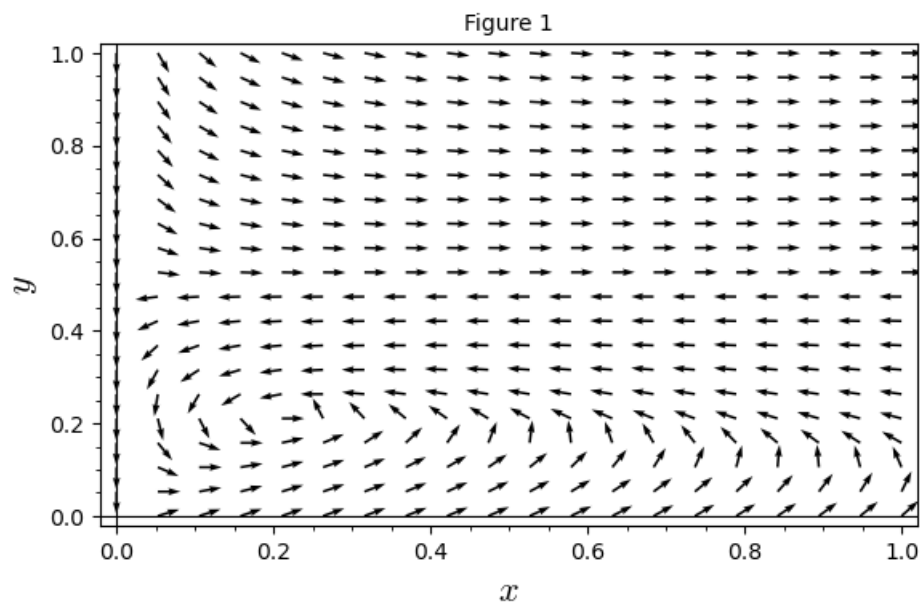

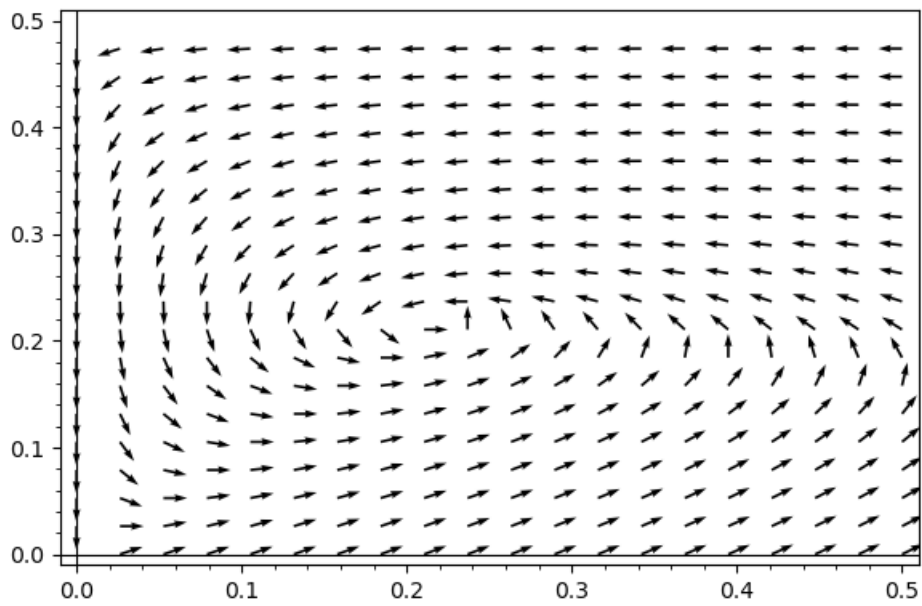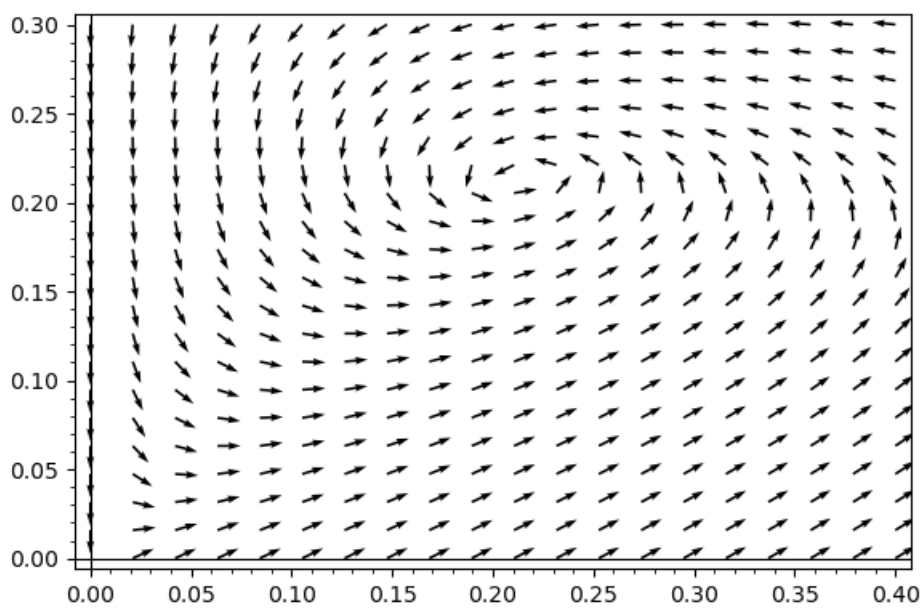

```
In [6]: plt1 = streamline_plot((vx,vy),(x,0,1),(y,0,1))
plt2 = streamline_plot((vx,vy),(x,0,.5),(y,0,.5))
plt3 = streamline_plot((vx,vy),(x,0,0.4),(y,0,.3))
show(plt1)
show(plt2)
show(plt3)
```

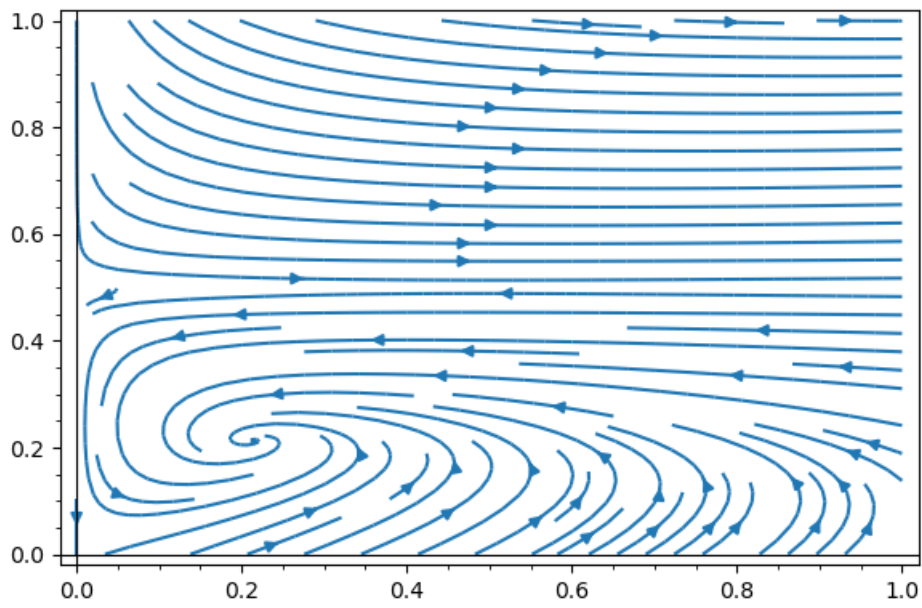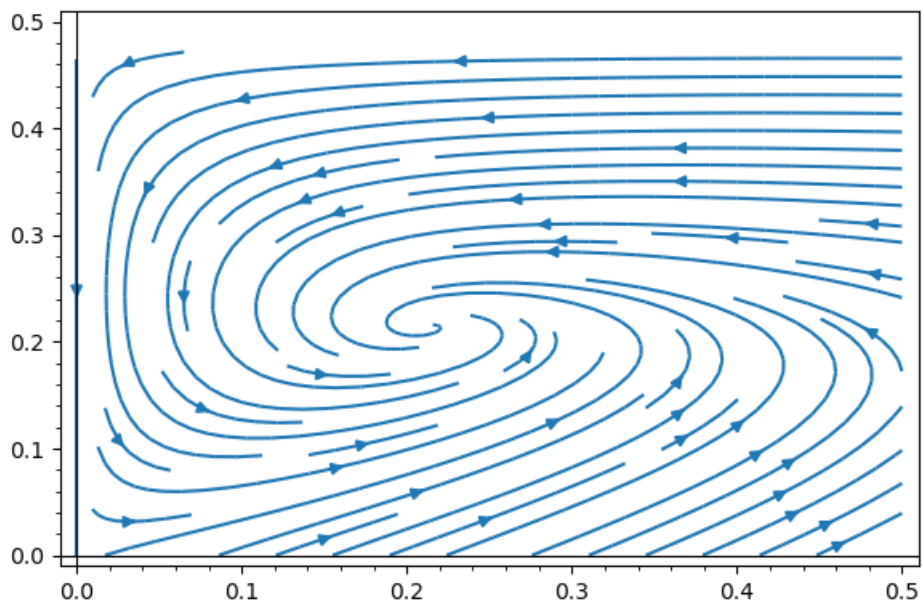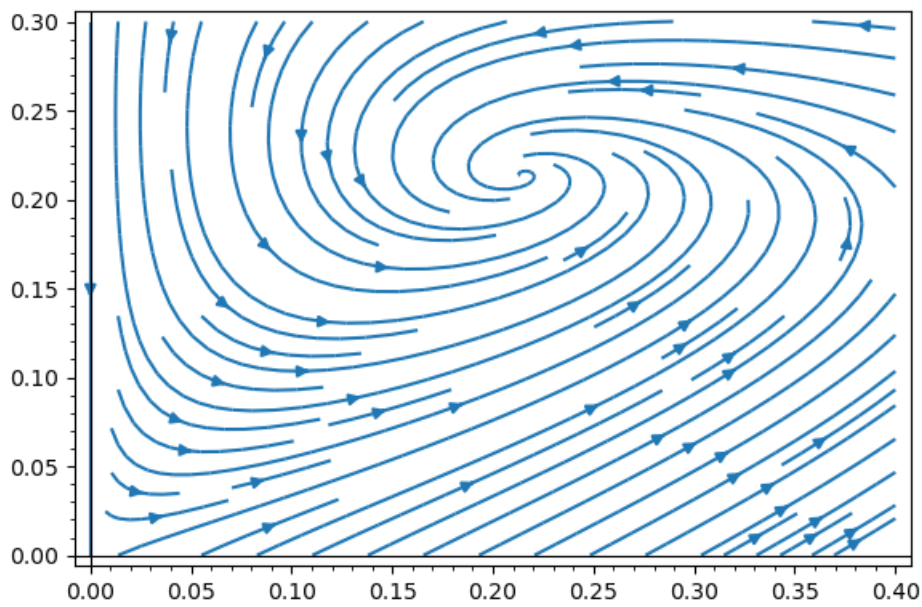

The solutions regular at  $r = 0$

Suppose  $\rho = \rho_0$  at  $r = 0$ . Then in the limit  $r \rightarrow 0$

$$m \rightarrow \frac{4}{3}\pi r^3 \rho_0 \quad x \rightarrow 4\pi G r^2 \rho_0 \quad y \rightarrow \frac{1}{3}x$$

So all the solutions regular at  $r = 0$  are on the trajectory that leaves  $(0, 0)$  along the line  $y = \frac{1}{3}x$ .

Changing the initial condition  $\rho(0) \rightarrow e^s \rho(0)$  is expressed by "time" translation along the flow,  $\ln r \rightarrow \ln r + \frac{1}{2}s$

In [7]:

```
set_precision(20)
ode_tol = None
ode_degree = None
#
t = var('t')
xdot = lambda x,y: x*(2-(1+1/w)*(y+w*x)/(1-2*y))
ydot = lambda x,y: x-y
F = lambda t,y: [xdot(y[0],y[1]), ydot(y[0],y[1])]

t0 = mpf(-7)
F0 = mpf(1)
y0 = mp.exp(2*t0)*F0
y1 = y0/3
traj = mp.odefun(F,t0,[y0,y1],tol=ode_tol,degree=ode_degree)
#
trajlist0 = [traj(t) for t in mp.linspace(t0,-5,100)]
trajlist1 = [traj(t) for t in mp.linspace(-5,-3.5,100)]
trajlist2 = [traj(t) for t in mp.linspace(-3.5,0,100)]
trajlist3 = [traj(t) for t in mp.linspace(0,5,100)]
trajlist4 = [traj(t) for t in mp.linspace(5,10,100)]
trajplot=list_plot(trajlist0+trajlist1+trajlist2+trajlist3+trajlist4,marker=None,plotjoined=True)
#list_plot(trajlist0+trajlist1+trajlist2+trajlist3+trajlist4,marker='.')
plt=trajplot+vfplot
plt.axes_labels([r"$x$",r"$y$"])
show(plt,title="Figure 2")
#plt.save('Figure_2_vf.pdf',title="Figure 2", dpi=300)
```

mp.dps =20    mp decimal precision =21    sage decimal precision =24

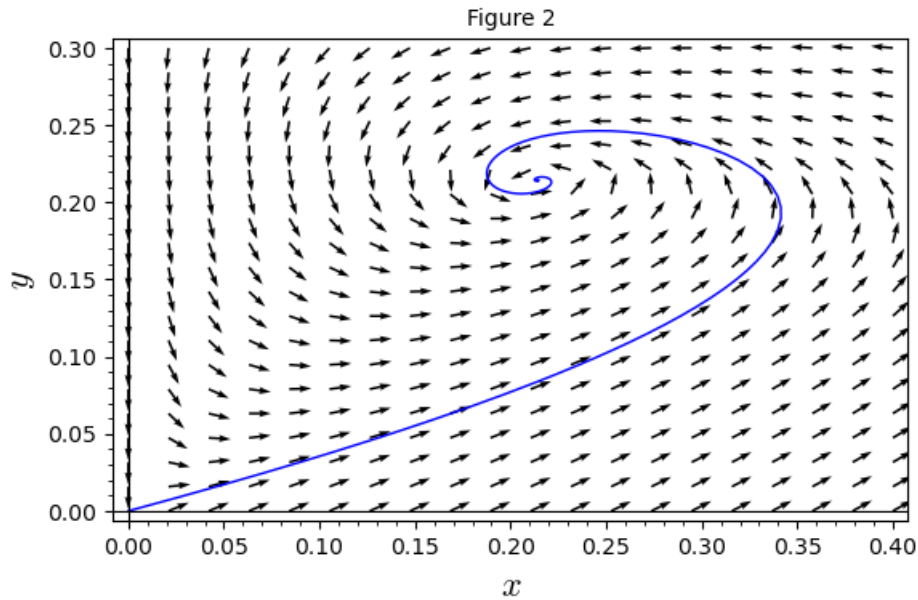

In [8]:

```
plt=trajplot+plt3
plt.axes_labels([r"$x$",r"$y$"])
show(plt,title="Figure 2")
#plt.save('Figure_2_vf.pdf',title="Figure 2", dpi=300)
```

Figure 2

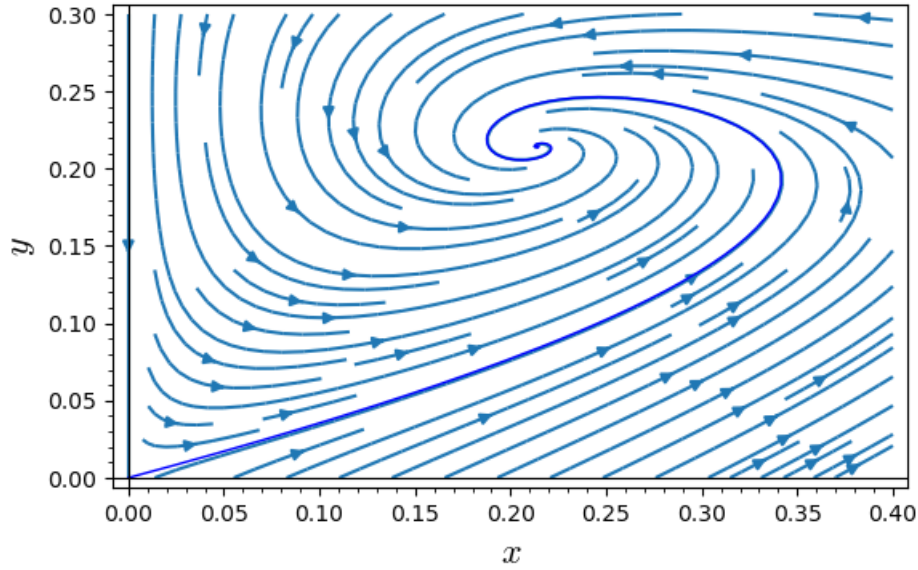

## $M$ - $R$ star curve

As the flow approaches the fixed point,  $r \rightarrow \infty$  with

$$\rho \rightarrow \frac{x_\infty}{4\pi G r^2} \quad m \rightarrow \frac{y_\infty r}{G}$$

The radius and mass are infinite because there is no cutoff at low density.

So introduce a cutoff at  $\rho_{min}$ . That is,  $\rho$  decreases to  $\rho_{min}$  with  $p = w\rho$ , then for  $\rho < \rho_{min}$ ,  $p = 0$ .

$$p = \begin{cases} w\rho & \rho > \rho_{min} \\ 0 & \rho \leq \rho_{min} \end{cases}$$

The stellar radius  $R$  is given by  $\rho(R) = \rho_{min}$ .

Parametrize the regular trajectory by  $t$  with

$$r \frac{d}{dr} = \frac{d}{dt} \quad \frac{dx}{dt} = 2x \frac{1 - (2+c)y - cw x}{1 - 2y} \quad \frac{dy}{dt} = x - y \quad c = \frac{1}{2} \left( 1 + \frac{1}{w} \right)$$

Let  $x(t), y(t)$  be the solution of the ode with initial condition

$$t \rightarrow -\infty \quad x(t) \rightarrow e^{2t} \quad y(t) \rightarrow \frac{1}{3} e^{2t}$$

Write the original change of variables as

$$\sqrt{4\pi G \rho} r = x^{1/2} \quad \sqrt{4\pi G^3 \rho} m = x^{1/2} y$$

and define dimensionless variables

$$\hat{r} = \sqrt{4\pi G \rho_{min}} r \quad \hat{m} = \sqrt{4\pi G^3 \rho_{min}} m$$

There is a solution with radius  $\hat{R}$  and mass  $\hat{M}$  iff for some  $t$

$$\hat{R} = x(t)^{1/2} \quad \hat{M} = x(t)^{1/2} y(t)$$

So the star curve in the  $\hat{M}$ - $\hat{R}$  plane is

$$t \mapsto \hat{M}(t), \hat{R}(t) = x(t)^{1/2} y(t), x(t)^{1/2}$$

The central density  $\rho(0)$  is a function of  $t$ . In the limit  $t' \rightarrow -\infty$ ,

$$r = Re^{t'-t} \quad \sqrt{4\pi G\rho}r = x(t')^{1/2} \quad \sqrt{4\pi G\rho}Re^{t'-t} \rightarrow e^{t'} \quad \sqrt{4\pi G\rho(0)}\frac{\hat{R}(t)}{\sqrt{4\pi G\rho_{min}}}e^{-t} = 1$$

$$\rho(0) = \rho_{min} \frac{e^{2t}}{\hat{R}(t)^2}$$

In [9]:

```
def MR(t):
    [x,y]=traj(t)
    xsqrt = sqrt(x)
    return [xsqrt*y,xsqrt]
MRlist = [MR(t) for t in mp.linspace(t0,5,100)]
plt = list_plot(MRlist,marker=None,plotjoined=True)
plt.axes_labels([r"$\hat{M}=x^{1/2} y$",r"$\hat{R}=x^{1/2}$"])
show(plt)
```

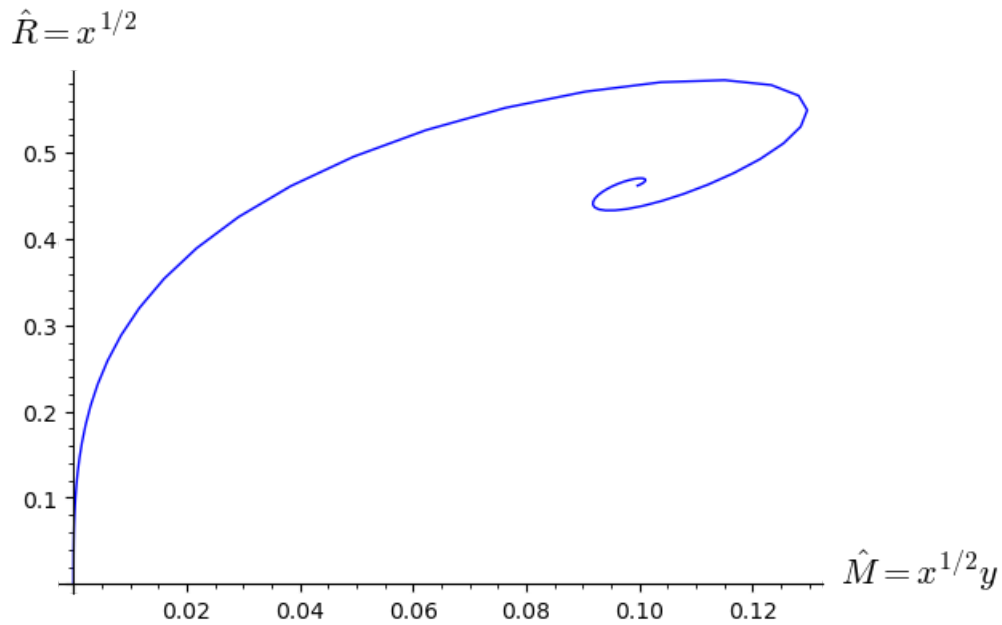

The curve near the fixed point is universal, independent of the low density cutoff.  
Away from the fixed point, the curve depends on the cutoff.
